# Supplementary material for: The Dipole of the Astrophysical Gravitational-Wave Background
Source: arXiv:2206.02747 source file (2022-12-05)
Supplement: Supplementary file 1 [file Noise.tex]

%\subsubsection{Instrumental Noise}
\label{Instrumental Noise}
If we consider BBH mergers in the mass range of $5-50\, M_\odot$, the most promising candidate to detect the anisotropies of this AGWB is a detector obtained by the combination of ET and CE, because
with the current bounds on the amplitude of the AGWB monopole, $\bar{\Omega}_{\rm AGWB}<3.4\times 10^{-9}$~\cite{KAGRA:2021kbb}, aLIGO has a too low sensitivity. Therefore, from now on, we will focus on the ET+CE case only. \DB{mettere referenze}\\
We have computed the angular power spectrum of the noise for the interferometers in the following configuration:
\begin{itemize}
\item we have considered the PSD of ET-D as shown in Figure \ref{all_noises_figure}. We have also considered a constant correlation matrix between different detectors\footnote{{\color{red}If we want to compute rigorously the correlation matrix, more time is needed.}}, 
\begin{equation}
N^{\rm ET} = N_{d}^{\rm ET} 
\begin{pmatrix}
1 & -\frac{1}{2} & -\frac{1}{2} \\
-\frac{1}{2} & 1 & -\frac{1}{2} \\
-\frac{1}{2} & -\frac{1}{2} & 1 
\end{pmatrix}\, .
\label{corr_matrix_et}
\end{equation}
Concerning the position of ET, we have considered ET in Sardinia, with latitude $40.1^\circ$ and longitude $9.0^\circ$.
\item The PSDs of the two CE interferometers are depicted in Figure \ref{all_noises_figure} too. We have considered no-correlation between the two CE detectors. We have also considered the two interferometers in Handford and Livingstone as for aLIGO\footnote{{\color{red} I don't know how the position of CE can affect the angular power spectrum of the noise, especially when combined with ET. For the moment, I don't have find a precise location of CE, so I have used the default one for LIGO provided by Schnell.}}.
\item We have used the following noise matrix for the combination of ET and CE,
\begin{equation}
N^{\rm ET+CE} = \begin{pmatrix}
N^{\rm ET} & 0 & 0 \\
0 & N^{\rm CE} & 0 \\
0 & 0 & N^{\rm CE}
\end{pmatrix}\, ,
\end{equation}
where $N^{\rm ET}$ is the $3\times 3$ matrix defined in Eq. \eqref{corr_matrix_et}.
\end{itemize}
To compute the angular power spectrum of the noise we have modified the public code Schnell~\cite{Alonso:2020rar}, finding $N_\ell^{\rm ET}$, $N_\ell^{\rm CE}$, and $N_\ell^{\rm ET+CE}$. The result is depicted in Figure \ref{detector_noise_figure} for $T_{\rm obs} = 10 \, \rm yr$. Remember that this noise refers to $\delta\rho_{\rm GW}$, while we evaluate the angular power spectrum in terms of $\delta_{\rm GW}=\delta\rho_{\rm GW}/\bar{\rho}_{\rm GW}$, therefore in the SNR computation we will divide the angular power spectrum of the noise derived here by the monopole squared of the AGWB considered.
\begin{figure}
\centering
\includegraphics[scale=0.45]{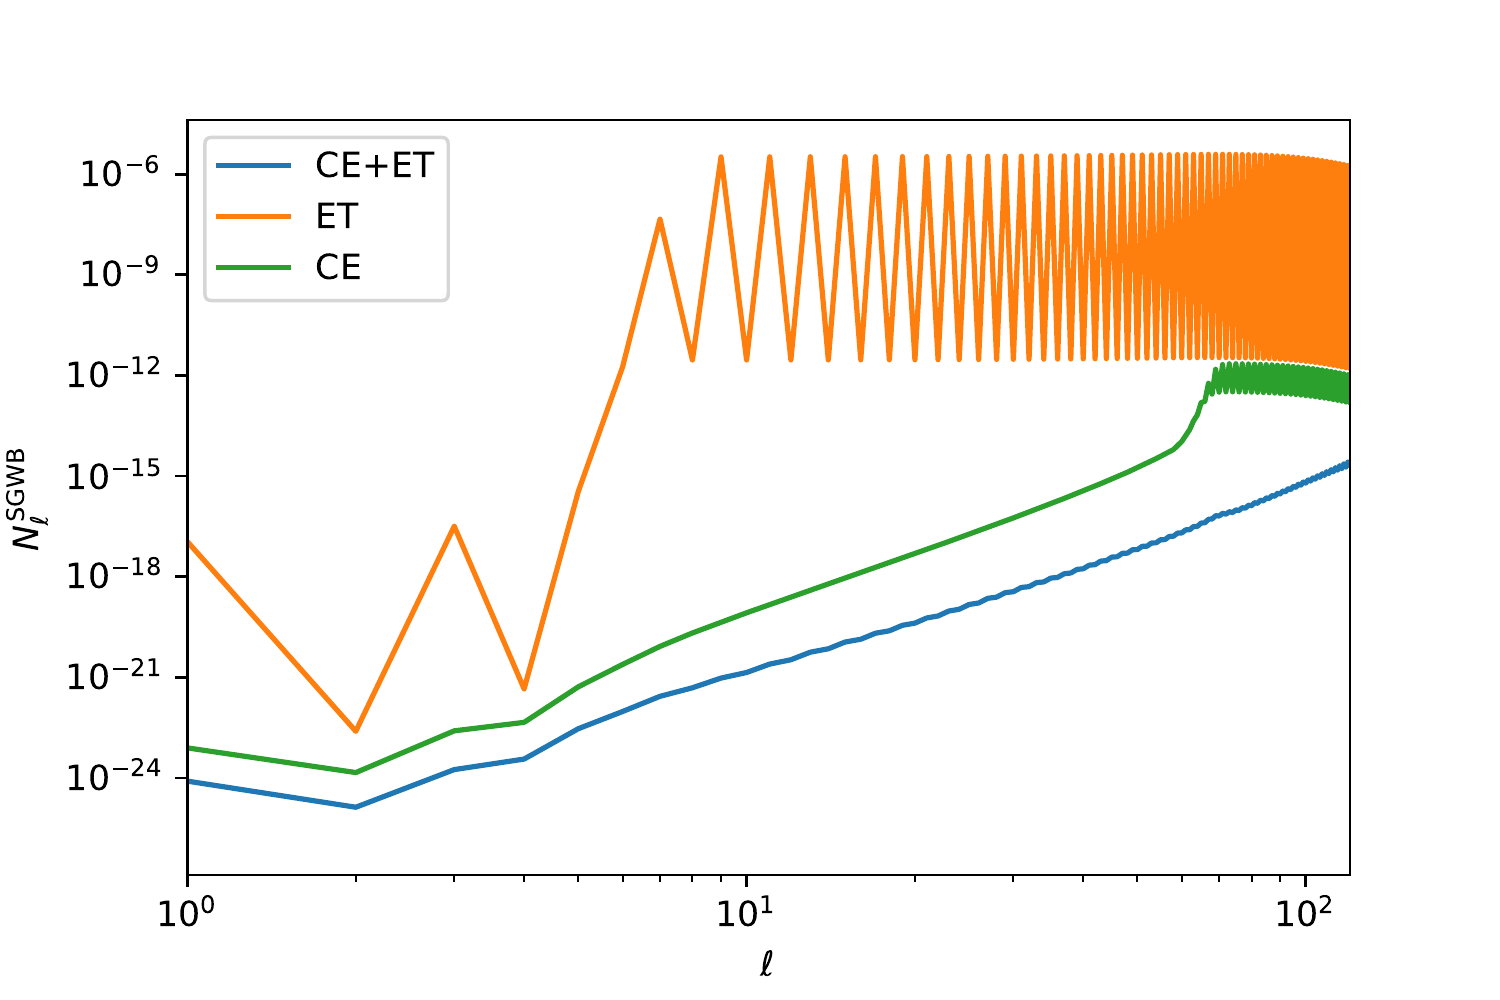}
\caption{Left: PSD of the angular power spectrum of the noise for ET, CE, and the combination of the two.}
\label{detector_noise_figure}
\end{figure}
