# Supplementary material for: The Dipole of the Astrophysical Gravitational-Wave Background
Source: arXiv:2206.02747 source file (2022-12-05)
Supplement: Supplementary file 4 [file appendix_aps_error.tex]

\label{Appendix_error_aps}
In this appendix we want to perform a detailed computation of the error associated to the estimators of the angular power spectra of the auto- and of the cross-correlation of two observables $a$ and $\Gamma$\footnote{We use $a$ and $\Gamma$ to relax the notation, but the only two fields we are interested in our work are the galaxy overdensity and the AGWB density contrast.}. We consider Gaussian random fields and we decompose them in spherical harmonics, ending up with $2(2\ell+1)$ Gaussian independent random variables, $\Gamma_{\ell m}$, $a_{\ell m}$, one for each value of $m$ at a fixed $\ell$. \\
The angular power spectra we are interested in are
\begin{equation}
\begin{split}
\langle a_{\ell m}\,a_{\ell^\prime m^\prime}^*\rangle \equiv&\delta_{\ell \ell^\prime}\delta_{m m^\prime} C_\ell^{aa}\, ,\\
\langle \Gamma_{\ell m}\,\Gamma_{\ell^\prime m^\prime}^*\rangle \equiv&\delta_{\ell \ell^\prime}\delta_{m m^\prime} C^{\Gamma\Gamma}_\ell\,,\\
\langle a_{\ell m}\,\Gamma_{\ell^\prime m^\prime}^*\rangle \equiv&\delta_{\ell \ell^\prime}\delta_{m m^\prime} C^{a\Gamma}_\ell\,.
\end{split}
\label{a_gamma_spectra_equation}
\end{equation}
Note that if we include the noise (instrumental noise, shot noise, or any kind of noise), the observed signals are
\begin{equation}
\begin{split}
s^\Gamma_{\ell m} = & \Gamma_{\ell m} + n^\Gamma_{\ell m}\, , \\
s^a_{\ell m}=& a_{\ell m} + n^a_{\ell m}\, .
\end{split}
\end{equation}
The noise has zero mean and we assume that it is Gaussian, therefore we can characterize it in terms of its angular power spectrum\footnote{In the case of the instrumental noise of a GW interferometer this is just an approximation, because the detector response function depends in general on the direction of observation.}
\begin{equation}
\begin{split}
\langle n_{\ell m}^X \rangle \equiv & 0\, ,  \\
\langle n_{\ell m}^X \, n_{\ell^\prime m^\prime}^{Y\, *} \rangle \equiv &  N_\ell^{XY}\, .
\end{split}
\end{equation}
Here we consider noises which are uncorrelated with the cosmological signals. Note that we cannot say apriori that the noises of two different experiments are uncorrelated, since sometimes there could be foregrounds which could be correlated. For example the SN between the galaxy oversendity and the AGWB density contrast are not independent, because fluctuations in the galaxy number in a volume $\delta V$ influence fluctuations in the number of GW sources in the volume $\delta V$, therefore there could be a non-negligible SN cross-term $N_\ell^{a \Gamma}$.

The statistical estimators of the angular power spectra of Eq. \eqref{a_gamma_spectra_equation} are the averages of the $2\ell+1$ angular power spectra we measure (the pseudo-$C_\ell$). For a generic combination of the two fields $x$, $y$ the estimator of the angular power spectrum $\hat{C}_\ell^{xy}$ is 
\begin{equation}
\begin{split}
\hat{C}_\ell^{xy} \equiv &\frac{1}{2\ell+1} \sum_{m=-\ell}^{\ell} s^x_{\ell m}s^{y\, *}_{\ell m}-N_\ell^{xy}\, . 
\end{split}
\end{equation}
The estimator we have introduce is unbiased,
\begin{equation}
\begin{split}
\langle \hat{C}_\ell^{xy}\rangle = C_\ell^{xy}\, .
\end{split}
\label{Eq_mean_estimator}
\end{equation}
The covariance matrix of the angular power spectrum is a block-diagonal matrix\footnote{We are assuming $f_{\rm sky}=1$, thus our covariance matrices are diagonal in the multipole $\ell$ because we have no mode coupling in this case.}, where each block contains contributions both from noise and cosmic variance. To compute it we use the Wick theorem for Gaussian random variables with zero mean, see e.g. Eq. (A1) of~\cite{Bloomfield:2018oku}, and a procedure analogue to the one used in~\cite{Knox:1994qj}. The variances of the auto-spectra of the pseudo-$C_\ell$ is simply
\begin{equation}
\begin{split}
    {\rm cov}\left(\hat{C}_\ell^{x y},\hat{C}_{\ell^\prime}^{x^\prime y^\prime}\right)=&\langle \left(\hat{C}_\ell^{xy}-C_\ell^{xy}\right)\left(\hat{C}_{\ell^\prime}^{x^\prime y^\prime}-C_{\ell^\prime}^{x^\prime y^\prime}\right)\rangle = \sum_{m,m^\prime}\frac{\left\langle s_{\ell m}^{xy}s_{\ell m}^{xy \, *}s_{\ell^\prime m^\prime}^{x^\prime y^\prime}s_{\ell^\prime m^\prime}^{x^\prime y^\prime \, *}\right\rangle}{(2\ell+1)^2}+N_\ell^{x y}N_{\ell^\prime}^{x^\prime y^\prime}+\\
    &+\left[-N_\ell^{xy}\left(N_{\ell^\prime}^{x^\prime y^\prime}+C_{\ell^\prime}^{x^\prime y^\prime}\right)-N_{\ell^\prime}^{x^\prime y^\prime}\left(N_{\ell}^{x y}+C_{\ell}^{xy}\right)\right]-C_\ell^{xy}C_{\ell^\prime}^{x^\prime y^\prime} = \\
    = & \left(C^{xy}_\ell+N^{xy}_\ell\right)\left(C_{\ell^\prime}^{x^\prime y^\prime}+N_{\ell^\prime}^{x^\prime y^\prime}\right)+\\
    &+\delta_{\ell \ell^\prime}\frac{\left[\left(C_\ell^{x y^\prime}+N_\ell^{x y^\prime}\right)\left(C_\ell^{y x^\prime}+N_\ell^{y x^\prime}\right)+\left(C_\ell^{x x^\prime}+N_\ell^{x x^\prime}\right)\left(C_\ell^{y y^\prime}+N_\ell^{y y^\prime}\right)\right]}{2\ell+1}+ \\
    &+(-1)\left[-N_\ell^{xy}\left(N_{\ell^\prime}^{x^\prime y^\prime}+C_{\ell^\prime}^{x^\prime y^\prime}\right)-N_{\ell^\prime}^{x^\prime y^\prime}\left(N_{\ell}^{x y}+C_{\ell}^{xy}\right)-C_\ell^{xy}C_{\ell^\prime}^{x^\prime y^\prime} \right]= \\
    = & \delta_{\ell \ell^\prime}\frac{\left[\left(C_\ell^{x y^\prime}+N_\ell^{x y^\prime}\right)\left(C_\ell^{y x^\prime}+N_\ell^{y x^\prime}\right)+\left(C_\ell^{x x^\prime}+N_\ell^{x x^\prime}\right)\left(C_\ell^{y y^\prime}+N_\ell^{y y^\prime}\right)\right]}{2\ell+1}\, .
\end{split}
\end{equation}
