# Supplementary material for: The Dipole of the Astrophysical Gravitational-Wave Background
Source: arXiv:2206.02747 source file (2022-12-05)
Supplement: Supplementary file 5 [file appendix_miny_window.tex]

\label{Detector Efficiency}
The detector efficiency is defined as the number of detected events divided by the total incoming events. This quantity is related to the rate of detected events at a given redshift with a SNR large enough to reject the null hypothesis. The value of the threshold depends on the detector, here we have chosen for the network of ET+CE the conservative value $\bar{\rho}=12$~\cite{Maggiore:2019uih}. \\
For Gaussian and stationary noise, the otpimal matched filtering SNR ($\rho$) is defined as~\cite{Finn:1995ah}
\begin{equation}
\rho^2 = 4\int_0^\infty df\, \frac{|h(f)|^2}{S_n(f)}\, ,
\end{equation}
where $S_n(f)$ is the one-sided PSD of the noise, and $h(f)$ is the Fourier transform of the detector response to GWs. \\
We assume that the amplitude of GWs is given by the quadrupolar formula\footnote{Of course we should include all the stages of the binary evolution, but for simplicity here we will consider only the inspiral phase, and we will generalize the expression in the final result only.}
\begin{equation}
|h(f)| = \frac{1}{D_L} \left(\frac{5}{24}\right)^{1/2}\left(\frac{M_z^5}{\pi^4}\right)^{1/6}\frac{\Theta}{4}f^{-7/6}\, ,
\end{equation}
where we have introduced the orientation function $\Theta$,
\begin{equation}
\Theta \equiv 2[F_+^2(1+\cos^2 i)^2+4F_\times^2 \cos^2 i]^{1/2}\, ,
\end{equation}
with $F_+$, $F_\times$ the detector's responses to different GW polarizations,
\begin{equation}
\begin{split}
F_+\equiv &  \frac{1}{2}(1+\cos^2\theta)\cos(2\phi)\cos(2\psi)-\cos\theta\sin(2\phi)\sin(2\psi)\, , \\
F_\times\equiv & \frac{1}{2}(1+\cos^2\theta)\cos(2\phi)\sin(2\psi)-\cos\theta\sin(2\phi)\cos(2\psi)\, .
\end{split}
\end{equation}
$\{\theta,\phi\}$ are the usual spherical coordinates for the direction of the binary relative to the detector, while $\{i,\psi\}$ describe the binary orientation w.r.t. the line-of-sight. More explicitly, if the arms of the detectors are identified by the directions $\{\hat{x},\hat{y}\}$, the remaining direction ortoghonal to both of them is $\hat{z}$, and if the position of the binary is identified with $\hat{n}$, we have 
\begin{equation}
\begin{split}
\cos\theta \equiv & -\hat{n}\cdot \hat{z}\, , \\
\tan\phi \equiv & \frac{\hat{n}\cdot \hat{y}}{\hat{n}\cdot \hat{x}}\, .
\end{split}
\end{equation}
If we identify with $\vec{J}$ the angular momentum of the binary we have 
\begin{equation}
\begin{split}
\cos i \equiv & -\frac{\vec{J}\cdot \hat{n}}{\left | \vec{J} \right |}\, , \\
\cot \psi \equiv & \frac{\vec{J}\cdot (\hat{n}\times \hat{z})}{\vec{J}\cdot [\hat{z}-\hat{n}(\hat{z}\cdot \hat{n})]}\, .
\end{split}
\end{equation}
It is clear that the PDF of the SNR depends on the astrophysical parameters and on the binary orientation. Here we want to focus on the angular dependence of the SNR. We can take uniform distributions between $-1$ and $+1$ for $\cos\theta$, $\phi/\pi$, $\cos i$, and $\psi/\pi$. By taking this prior, it has been shown that the PDF is~\cite{Finn:1992xs}
\begin{equation}
P_\Theta(\Theta)= \begin{cases}
5\Theta(4-\Theta)^3/256 \hspace{2.3em} 0<\Theta < 4 \\
0 \hspace{9em} \rm otherwise
\end{cases}
\end{equation}
To find the detector efficiency we use the change of variables from $\rho$ to $\Theta$:
\begin{equation}
p(\rho)d\rho = P_\Theta(\Theta)d\Theta\rightarrow p(\rho)=P_\Theta(\Theta)\frac{1}{\frac{d\rho}{d\Theta}}\, ,
\end{equation}
with
\begin{equation}
\begin{split}
\rho(\Theta)=& \sqrt{4\int_0^\infty df\, \left[\frac{1}{D_L} \left(\frac{5}{24}\right)^{1/2}\left(\frac{M_c^5}{(1+z)^5\pi^4}\right)^{1/6}\frac{\Theta}{4}f^{-7/6}\right]^2\frac{1}{S_n(f)}}\propto \frac{\Theta}{D_L}\left(\frac{M_c}{(1+z)}\right)^{5/6}\, .
\end{split}
\end{equation}
The probability distribution of the SNR depends on the chirp mass $M_{\rm c}$ of the source of the GWs, on the mass ratio $q$ of the compact objects that form the binary, and on the redshift $z$ at which the event occurred. \\
According to~\cite{Taylor:2012db,Boco:2019teq}, the full expression we will plug in is
\begin{equation}
\Theta_\rho =  \frac{\rho}{8}\frac{D_L(z)}{R_0}\left[\frac{1.2\, M_{\odot}}{(1+z)M_{\rm c}}\right]^{5/6}\frac{1}{\sqrt{\zeta_{\rm isco}+\zeta_{\rm insp}+\zeta_{\rm merg}+\zeta_{\rm ring}}}\, ,
\label{theta_rho_equation}
\end{equation}
where $R_0$ is the characteristic distance parameter, and the $\zeta$ functions specify the overlap of the waveform with the observational bandwidth during different phases of the event. \\
The characteristic distance parameter depends on the detector considered and it can be computed by using
\begin{equation}
R_0^2=\frac{5M^2_{\odot}}{192\pi c^3}\left(\frac{3G}{20}\right)^{5/3}x_{7/3}\, , 
\end{equation}
where $x_{7/3}$ is an auxiliary function which depends on the PSD of the detector $S(f)$ through
\begin{equation}
x_{7/3}=\int_0^{\infty} df \frac{1}{(\pi M_\odot)^{1/3} f^{7/3} S(f)}\, .
\end{equation}
Numerical examples of the characteristic distance parameter for different detectors can be found in Table 1 of~\cite{Taylor:2012db}. For instance, for ET-D, $R_0= 1591\, \rm Mpc$. \\
For all the stages of binary evolution we have
\begin{equation}
\begin{split}
\zeta_{\rm isco}=&\frac{1}{(\pi M_{\odot})^{1/3}x_{7/3}}\int_0^{2 f_{\rm isco}}\frac{df}{S(f)}\frac{1}{f^{7/3}}\, , \\
\zeta_{\rm insp}=&\frac{1}{(\pi M_{\odot})^{1/3}x_{7/3}}\int_{2 f_{\rm isco}}^{f_{\rm merg}} \frac{df}{S(f)}\frac{1}{f^{7/3}}\, , \\
\zeta_{\rm merg}=&\frac{1}{(\pi M_{\odot})^{1/3}x_{7/3}}\int_{ f_{\rm merg}}^{f_{\rm ring}} \frac{df}{S(f)}\frac{1}{f_{\rm merg}f^{4/3}}\, , \\
\zeta_{\rm ring}=&\frac{1}{(\pi M_{\odot})^{1/3}x_{7/3}}\int_{ f_{\rm ring}}^{f_{\rm cut}}\frac{df}{S(f)}\frac{1}{f^{7/3}}\left[1+\left(\frac{f-f_{\rm ring}}{\sigma_{\rm ring}/2}\right)^2\right]^{-2}\, .
\end{split}
\end{equation}
Our final PDF is
\begin{equation}
P(\rho)=P_\Theta(\Theta)\frac{\Theta}{\rho}.
\end{equation}
The window function $w(z)$, equal to 1 minus the detector efficiency, is defined as the probability of having an SNR smaller than the threshold of the detection of a resolved source,
\begin{equation}
w(z)= \int_{\Theta(0)}^{\Theta(\rho_{\rm threshold})} d\Theta \, P_\Theta(\Theta)\frac{\Theta}{\rho(\Theta)}\, .
\end{equation}
