# Supplementary material for: The Dipole of the Astrophysical Gravitational-Wave Background
Source: arXiv:2206.02747 source file (2022-12-05)
Supplement: Supplementary file 6 [file Estimator.tex]

Now we want to generalize the previous computation to derive the best unbiased estimator for the AGWB kinematic dipole, keeping into account also the instrumental noise. To combine SN and instrumental noise, we use the code Schnell, therefore here we will use the same formalism of~\cite{Alonso:2020rar}. The AGWB is described by 
\begin{equation}
h_{ij}(t,\vec{x}) = \sum_{p} \int df \int d\hat{n}\, h_p(f,\hat{n})e^{2\pi i f (t-\hat{n}\cdot \vec{x})}e_{ij}^p(\hat{n})\, ,
\end{equation}
where $p$ is the GW polarization and $\hat{n}$ the direction of observation. The response of a detector $A$ at position $\vec{x}_A$ for an observation time $T$ is 
\begin{equation}
d_{A,T}(t,f) \simeq \int d\hat{n} \sum_p F_A^p(f,\hat{n}) h_p^{\rm tot}(f,\hat{n})+n_{A,T}\, ,
\label{data_definition}
\end{equation}
where we have introduced
\begin{equation}
F_A^p \equiv a_A^{ij}e_{ij}^p e^{-2\pi i f \hat{n}\cdot \vec{x}_A}\, ,
\end{equation}
with $a_A^{ij}$ the detector response function. Note that for the AGWB $h_p^{\rm tot}$ is the sum of three contributions,
\begin{equation}
h^{\rm tot}_p(f,\hat{n}) = h^{\rm KD}_p(f,\hat{n})+h^{\rm int}_p(f,\hat{n})+h^{\rm SN}_p(f,\hat{n})\, .
\end{equation}
The power spectrum of $h_p$ is 
\begin{equation}
\langle h_p(f,\hat{n})h_{p^\prime}^*(f^\prime,\hat{n}^\prime)\rangle \equiv \frac{1}{2}\delta(f-f^\prime)\frac{\delta(\hat{n}-\hat{n}^\prime)}{4\pi}\delta_{p p^\prime}I(f,\hat{n})\, ,
\end{equation}
where we have assumed that the only non-null Stokes parameter is the intensity, therefore we are legitimated to introduce $\delta_{p p^\prime}$. The amplitude of the SGWB is related to the intensity through
\begin{equation}
\Omega_{\rm GW}(f,\hat{n}) = \bar{\Omega}_{\rm GW}(f)\left[1+\delta_{\rm GW}(f,\hat{n})\right]= \frac{4\pi f^3}{3H_0^2} I(f,\hat{n})\, .
\label{I_Omega_Equation}
\end{equation}
As stressed in Section \ref{Kinematic dipole}, the frequency dependence of the AGWB kinematic dipole intensity can be factorized,
\begin{equation}
\begin{split}
I^{\rm KD}(\hat{n},f) =& \frac{\Omega_{\rm AGWB}(f)/f^3}{\Omega_{\rm AGWB}(f_{\rm piv})/f_{\rm piv}^3}\frac{C_\ell^{\rm AGWB,KD}(f,f_{\rm piv})}{C_\ell^{\rm AGWB,KD}(f_{\rm piv},f_{\rm piv})}I^{\rm KD}(\hat{n},f_{\rm piv})\\
= & \mathcal{E}^{\rm KD}(f,f_{\rm piv})I^{\rm KD}_{\rm piv}(\hat{n})\, ,
\end{split}
\end{equation}
where $\mathcal{E}^{\rm KD}(f,f_{\rm piv})$ is related to the ratio between the Kaiser-Rocket factors at two frequencies,
\begin{equation}
\mathcal{E}^{\rm KD}(f,f_{\rm piv})\equiv  \frac{\Omega_{\rm AGWB}(f)/f^3}{\Omega_{\rm AGWB}(f_{\rm piv})/f_{\rm piv}^3}\frac{\mathcal{R}(f)}{\mathcal{R}(f_{\rm piv})}\, .
\end{equation}
We plot the ratio between the Kaiser-Rocket factors and the factor $\mathcal{E}^{\rm KD}(f,f_{\rm piv})$ in Figure \ref{dipole_factors_figure}, for $f_{\rm piv}=50\, \rm Hz$.
Now we want to build an estimator for the kinematic dipole intensity $I_{\rm piv}^{\rm KD}(\hat{n})$, which is related to the velocity of our frame by
\begin{equation}
I_{\rm piv}^{\rm KD}(\hat{n}) = \mathcal{R}(f_{\rm piv})\,\hat{n}\cdot\vec{v}_o\,.
\end{equation}
So, once we have reconstructed the map, it is immediate to extract the dipole and then $\vec{v}_o$.
\begin{figure}
\includegraphics[scale=0.50]{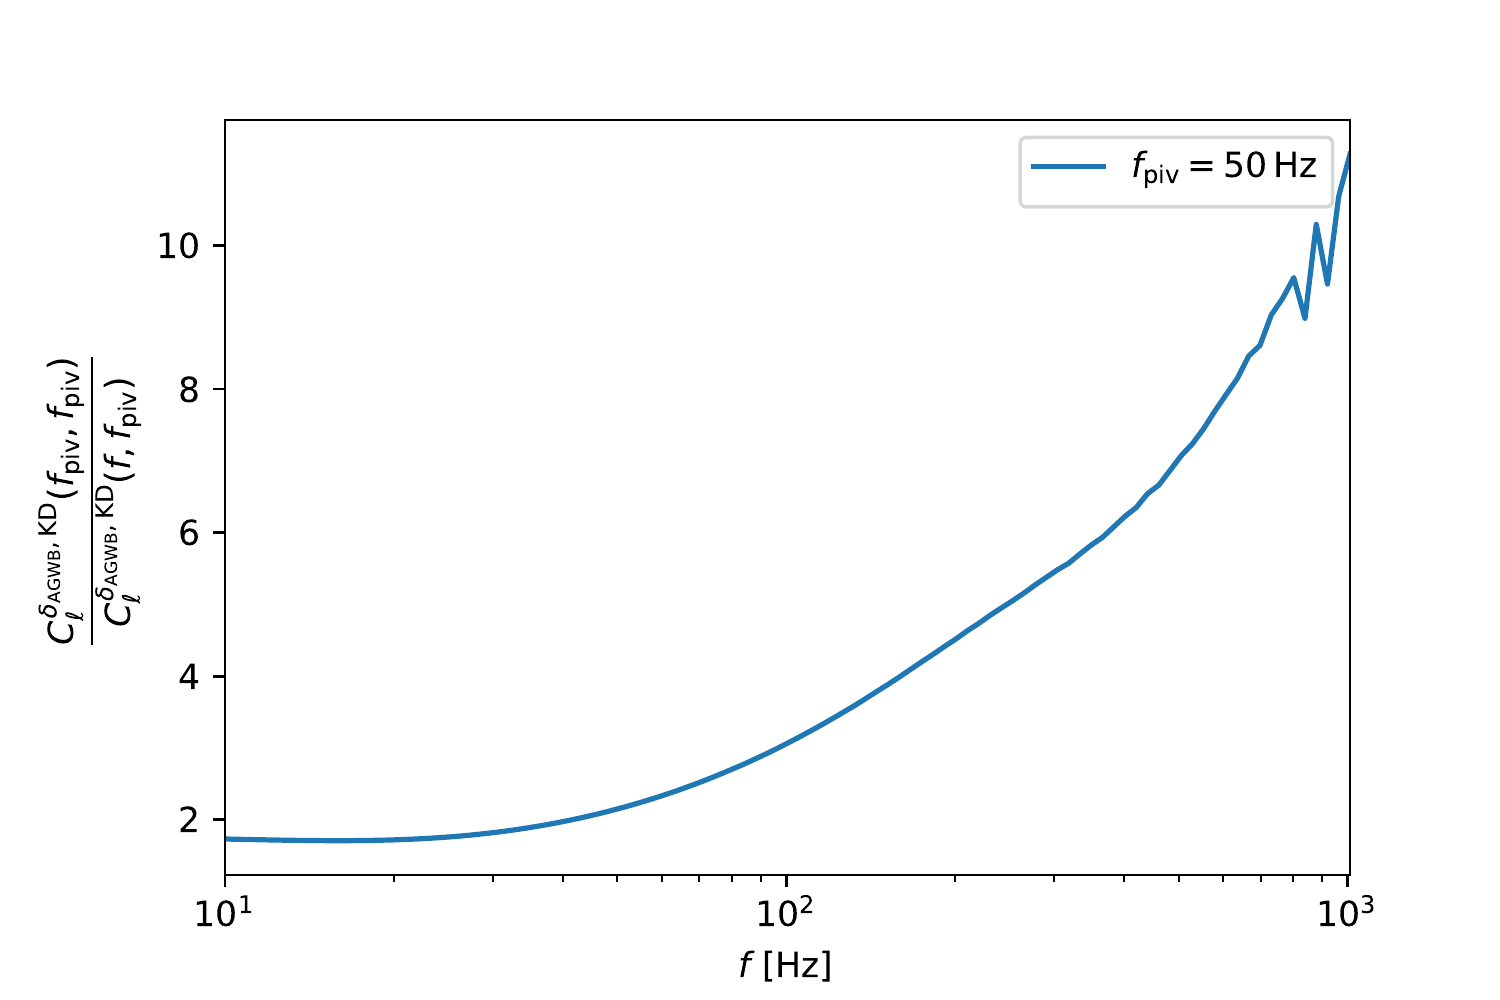}\includegraphics[scale=0.50]{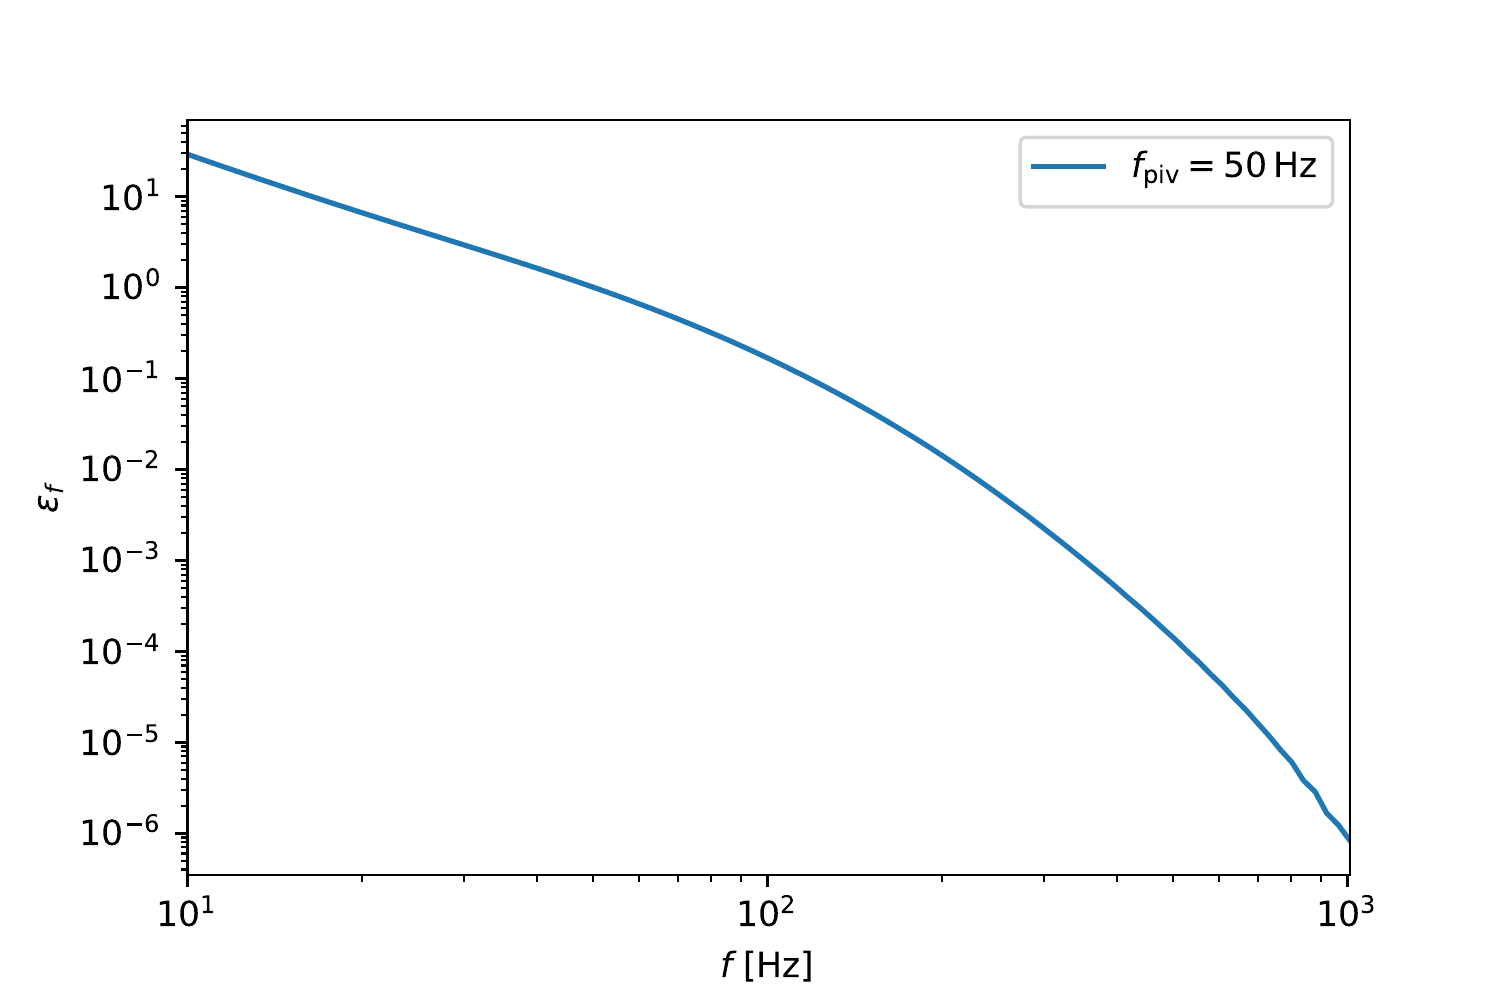}
\caption{Left: plot of the ratio between the Kaiser-Rocket factor of the kinematic dipole at frequencies $f$ and $f_{\rm piv}$. Note that the Kaiser-Rocket factor in this case is equal to the ratio between the angular power spectrum of the cross-correlation at $f$, $f_{\rm piv}$, divided by the angular power spectrum of the auto-correlation at $f_{\rm piv}$. This ratio increases at higher frequencies basically because of the behaviour of the evolution bias. Right: ratio between the intensity of the kinematic dipole at frequencies $f$ and $f_{\rm piv}$. In this case the behaviour of this ratio is due to the scaling with the frequency of the monopole $\bar{\Omega}_{\rm AGWB}(f)$.}
\label{dipole_factors_figure}
\end{figure}

When we perform component separation with ILC we build an estimator of the form {\color{red} Questo e' standard o e' quello che troviamo noi?}\\
\begin{equation}
\hat{d}_{\rm piv}^{\rm kin} = \frac{\vec{a}^TC^{-1}\vec{d}}{\vec{a}^TC^{-1}\vec{a}}\, ,
\end{equation}
where $\vec{d}$ are the measured dipoles in our maps. Since we want to include the instrumental noise too, the estimator cannot be built from GW density contrasts, but we have to start from the GW strain $h$. A linear estimator in the dipole corresponds to a quadratic estimator in the strain. In our case the optimal estimator for the kinematic dipole is a quadratic estimator,
\begin{equation}
\tilde{I}^{\rm KD}_{\rm piv,\theta} = \sum_{A,B,f,f^\prime} d_{f,A}E^{f f^\prime}_{\theta,AB}d_{f^\prime,B}-b_\theta\, ,
\end{equation}
where the matrix $E$ and the vector $b$ have to be determined by minimizing the covariance and by eliminating the bias. Even if we are working in pixel space, our discrete approach is consistent with~\cite{Mentasti:2020yyd,LISACosmologyWorkingGroup:2022kbp}.\\

The covariance matrix of the data, defined in Eq. \eqref{data_definition}, is 
\begin{equation}
\langle d_{f,A} d^*_{f^\prime,B}\rangle = \frac{1}{2}\frac{\delta_{f f^\prime}}{\Delta f}\left[N^{AB}_f+\sum_\theta B^{A B,\rm KD}_{f \theta}\left(I^{\rm KD}_{\rm piv,\theta}+\frac{I_{\theta,f}^{\rm int}+I_{\theta,f}^{\rm SN}}{\mathcal{E}_f^{\rm KD}}\right)\right]\, ,
\end{equation}
where $I^{\rm KD/int/SN}_{\theta}$ are the theoretical kinematic dipole/intrinsic/SN maps respectively, $N_f^{AB}$ is the Power Spectral Density (PSD) of the noise of the interferometers, while the matrix $B$ is
\begin{equation}
B_{f,\theta}^{AB,\rm KD} \equiv \Delta \Omega \, \mathcal{E}^{\rm KD}_f \sum_p F_{A,f\theta}^p F_{B,f\theta}^{p\,*}\, .
\end{equation}
The mean of the estimate that we have found is
\begin{equation}
\begin{split}
\langle \tilde{I}^{\rm KD}_{\rm piv,\theta} \rangle =& \sum_{A,B,f,f^\prime} \langle d_{f,A} d_{f^\prime,B}\rangle E^{f f^\prime}_{\theta,AB}-b_\theta =\\
= &  \sum_{A,B,f} \frac{1}{2\Delta f}E_{\theta,AB}^{ff}\sum_{\theta^\prime}B_{f,\theta^\prime}^{AB,\rm KD}\left(I_{\rm piv, \theta^\prime}^{\rm KD}+\frac{I_{f, \theta^{\prime}}^{\rm int}+I_{f, \theta^{\prime}}^{\rm SN}}{\mathcal{E}_f^{\rm KD}}\right)+\sum_{A,B,f} \frac{1}{2\Delta f}E_{\theta,AB}^{ff}N_f^{AB,\rm inst}-b_\theta\, ,
\end{split}
\end{equation}
from which it is clear that the bias has to be equal to
\begin{equation}
b_\theta = \sum_{A,B,f} \frac{1}{2\Delta f}\,E_{\theta,AB}^{ff}\,N_f^{AB,\rm inst}\, .
\end{equation}
The bias we have defined here depends on the instrumental noise only, while the bias given by the SN and by the intrinsic dipole is reduced by the $E^{f f^\prime}_\theta$ coefficients. More specifically, we will try to minimize the covariance associated to our estimator and this will give us the full expression for $E^{f f^\prime}_\theta$. \\
Note that our estimator $\tilde{I}^{\rm KD}_{\rm piv,\theta}$ is related to the true kinematic dipole $I^{\rm KD}_{\rm piv,\theta}$ by a matrix multiplication in pixel space, therefore, the truly unbiased estimator is
\begin{equation}
\hat{I}_{\rm piv,\theta}^{\rm KD} = \sum_{\theta^\prime}\left(M^{-1}\right)_{\theta\theta^\prime}\tilde{I}_{\rm piv,\theta^\prime}^{\rm KD}\, ,
\end{equation}
where the matrix $M$ is defined by
\begin{equation}
M_{\theta \theta^\prime} \equiv \sum_{A,B,f} \frac{1}{2\Delta f}E^{ff}_{\theta,AB}B_{f,\theta^\prime}^{AB,\rm KD}\, .
\end{equation}
As in the ILC case, we want an unbiased estimator, therefore we require that $\hat{I}_{\rm piv,\theta}^{\rm KD}\propto I_{\rm piv,\theta}^{\rm KD}$, which means that $M_{\theta \theta^\prime}$ is diagonal in pixel space, which implies that 
\begin{equation}
M_{\theta \theta^\prime} = \delta_{\theta \theta^\prime}\rightarrow \sum_{A,B,f} \frac{1}{2\Delta f}E^{ff}_{\theta,AB}B_{f,\theta^\prime}^{AB,\rm KD} = \delta_{\theta \theta^\prime}\, .
\end{equation}
Therefore, the mean value of our estimator can be written as
\begin{equation}
\langle\hat{I}_{\rm piv,\theta}^{\rm KD} \rangle = \langle \tilde{I}_{\rm piv,\theta}^{\rm KD}\rangle = I_{\rm piv,\theta}^{\rm KD}+\frac{1}{2\Delta f}\sum_{f,\theta^\prime}  {\rm Tr}\left(E^{ff}_\theta B_{f\theta^\prime}^{\rm KD}\right)\frac{I_{f, \theta^{\prime}}^{\rm int}+I_{f, \theta^{\prime}}^{\rm SN}}{\mathcal{E}_f^{\rm KD}}\, .
\end{equation}
The covariance of our estimator is computed w.r.t. the data $d_{A,f}$, but there are two different sources of covariance. The first source of error is given by the fact that the signal $h$ measured at interferometers has zero mean and covariance related to the intensity (monopole amplitude) of the stochastic background considered. This source of error has to be summed in quadrature with the error given by instrumental noise, which is supposed to be dominant in many scenarios, but not here, because we know that SN plays a significant role in the uncertainty of our measurement, therefore we will keep the covariance matrix as much general as possible. The covariance associated to fluctuations of the strain amplitude $h$ is computed assuming that the noise and the signal are Gaussian, therefore the four-point function of the strain can be written as the sum of the product of two-point functions,
\begin{equation}
\begin{split}
{\rm cov}\left(\hat{I}_{\rm piv,\theta}^{\rm KD},\hat{I}_{\rm piv,\theta^\prime}^{\rm KD}\right)_h=& \Biggl \langle \left(\frac{1}{2\Delta f} \sum_{f f^\prime,A,B}d_{f,A} E^{f f^\prime}_{\theta,AB}d_{f^\prime,B}-E^{f f^\prime}_{\theta,AB}\langle d_{f,A}d_{f^\prime,B}\rangle\right)\times 
\\ & \times
\left(\frac{1}{2\Delta f} \sum_{f^{\prime\prime} f^{\prime\prime\prime},C,D}d_{f^{\prime\prime},C} E^{f^{\prime\prime} f^{\prime\prime\prime}}_{\theta^\prime,CD}d_{f^{\prime\prime\prime},D}-E^{f^{\prime\prime} f^{\prime\prime\prime}}_{\theta^\prime,CD}\langle d_{f^{\prime\prime},C}d_{f^{\prime\prime\prime},D}\rangle\right) 
 \Biggl \rangle=\\
 = & \frac{1}{(2\Delta f)^2}\sum_{f ,f^\prime, f^{\prime\prime},f^{\prime\prime\prime}}E^{f f^\prime}_{\theta,AB}E^{f^{\prime\prime}f^{\prime\prime\prime}}_{\theta^\prime,CD}\left(\langle d_{f,A}d_{f^\prime,B}d_{f^{\prime\prime},C}d_{f^{\prime\prime\prime},D}\rangle-\langle d_{f,A}d_{f^\prime,B}\rangle\langle d_{f^{\prime\prime},C}d_{f^{\prime\prime\prime},D}\rangle\right)\, .
\end{split}
\end{equation}
Now we note that when we take the four-point function by coupling $A$ with $B$ and $C$ with $D$, we obtain a term that cancels the second one in the sum. If we define the total covariance matrix of the strain as
\begin{equation}
S_f^{AB} = N^{AB}_f+\sum_{\theta^\prime} B^{A B,\rm KD}_{f \theta^\prime}\left(I_{\rm piv, \theta^\prime}^{\rm KD}+\frac{I_{f, \theta^{\prime}}^{\rm int}+I_{f, \theta^{\prime}}^{\rm SN}}{\mathcal{E}_f^{\rm KD}}\right)\, ,
\end{equation}
we have that the covariance generated by fluctuations in $h$ is 
\begin{equation}
\begin{split}
{\rm cov}\left(\hat{I}_{\rm piv,\theta}^{\rm KD},\hat{I}_{\rm piv,\theta^\prime}^{\rm KD}\right)_h= & \frac{1}{(2\Delta f)^2}\sum_{f ,f^\prime, f^{\prime\prime},f^{\prime\prime\prime}}E^{f f^\prime}_{\theta,AB}E^{f^{\prime\prime}f^{\prime\prime\prime}}_{\theta^\prime,CD}\left(S_f^{AC}S_{f^\prime}^{BD}\delta_{f f^{\prime\prime}}\delta_{f^\prime f^{\prime\prime\prime}}+S_f^{AD}S_{f^\prime}^{BC}\delta_{f f^{\prime\prime\prime}}\delta_{f^\prime f^{\prime\prime}}\right)= \\
= &  \frac{1}{2\Delta f^2}\sum_{f,f^\prime}{\rm Tr}\left(S_f E_{\theta}^{f f^\prime}S_{f^\prime}E^{f^\prime f}_{\theta^\prime}\right)\, .
\end{split}
\end{equation}
\begin{figure}
\centering
\includegraphics[scale=0.5]{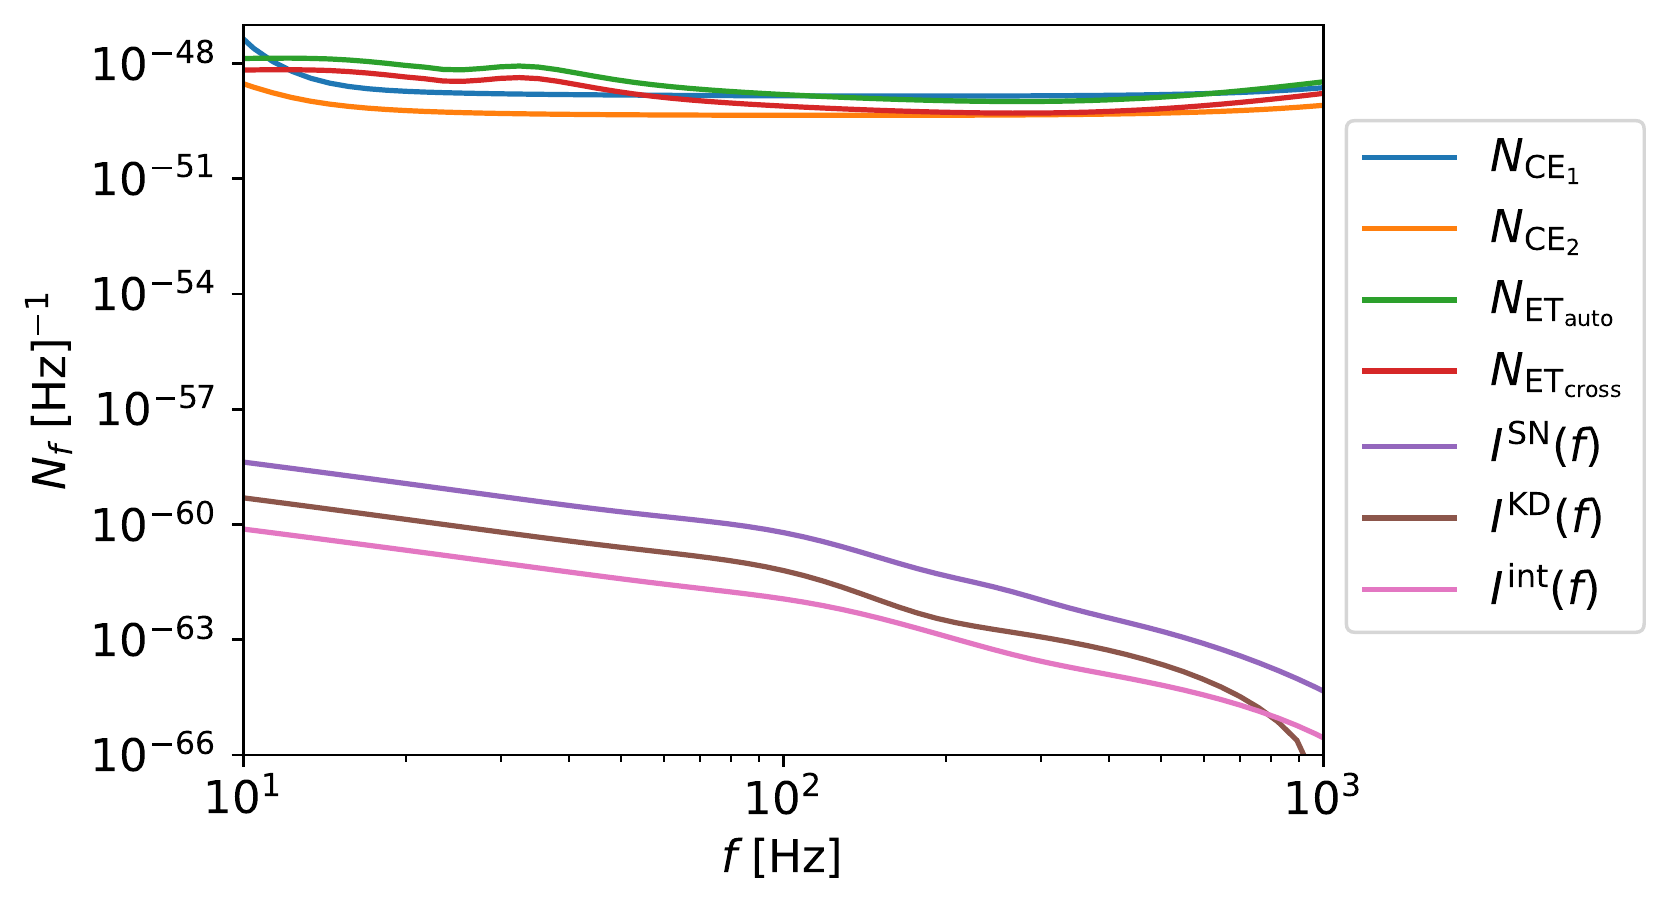}
\caption{PSDs of the noise of the detector ET, CE1, CE2, and of the possible cross-correlations between the ET channels. We have depicted also the intensity of the SN at different frequencies. Note that SN (and so the signal) are much smaller than instrumental noise, but with this (standard) technique, we are able to clean the signal a lot.}
\label{all_noises_figure}
\end{figure}
The contribution to the matrix $S_f$ are plotted in Figure \ref{all_noises_figure}.
There is another source of error in our estimator: here we are not trying to estimate just the total map $I_{\theta}^{\rm tot}$, but we are trying to perform component separation between different contributions in the map. This point is crucial, because in this step we want to quantify the amount of uncertainty in our measurement provided by the SN. In our analysis we have an estimate for the kinematic dipole $\hat{I}^{\rm KD}_{\rm piv,\theta}$ whose mean value $\langle \hat{I}^{\rm KD}_{\rm piv,\theta}\rangle$ differs from the true map $I_{\rm piv,\theta}^{\rm KD}$ because of SN and the intrinsic anisotropies. These fluctuations are quantified by cosmic variance and they can be computed in the following way,
\begin{footnotesize}
\begin{equation}
\begin{split}
{\rm cov}\left(\left\langle\hat{I}_{\rm piv,\theta}^{\rm KD}\right\rangle,\left\langle\hat{I}_{\rm piv,\theta^\prime}^{\rm KD}\right\rangle\right)_{cv} = & \left\langle \left(\langle \hat{I}^{\rm KD}_{\rm piv,\theta}\rangle_h - I^{\rm KD}_{\rm piv,\theta}\right) \left(\langle \hat{I}^{\rm KD}_{\rm piv,\theta^\prime}\rangle_h - I^{\rm KD}_{\rm piv,\theta^\prime}\right)\right\rangle_{cv} = \\
= & \left\langle \sum_{f,\theta^{\prime\prime}}\frac{1}{2\Delta f}{\rm Tr}\left(E^{ff}_{\theta}B^{\rm KD}_{f \theta^{\prime\prime}}\right)\frac{I_{f, \theta^{\prime\prime}}^{\rm int}+I_{f, \theta^{\prime\prime}}^{\rm SN}}{\mathcal{E}_f^{\rm KD}}\sum_{f^\prime,\theta^{\prime\prime\prime}}\frac{1}{2\Delta f}{\rm Tr}\left(E^{f^\prime f^\prime}_{\theta^\prime}B^{\rm KD}_{f^\prime \theta^{\prime\prime\prime}}\right)\frac{I_{f^\prime, \theta^{\prime\prime\prime}}^{\rm int}+I_{f^\prime, \theta^{\prime\prime\prime}}^{\rm SN}}{\mathcal{E}_{f^\prime}^{\rm KD}}\right\rangle = \\
= & \frac{1}{(2\Delta f)^2}\sum_{f,f^\prime,\theta^{\prime\prime}\theta^{\prime\prime\prime}}{\rm Tr}\left(E^{ff}_\theta B^{\rm KD}_{f \theta^{\prime\prime}}\right){\rm Tr}\left(E^{f^\prime f^\prime}_{\theta^\prime} B^{\rm KD}_{f^\prime \theta^{\prime\prime\prime}}\right)\frac{C_{f f^\prime,\theta^{\prime\prime}\theta^{\prime\prime\prime}}^{\rm int}+C_{f f^\prime,\theta^{\prime\prime}\theta^{\prime\prime\prime}}^{\rm SN}}{\mathcal{E}_f^{\rm KD}\mathcal{E}_{f^\prime}^{\rm KD}}\, ,
\end{split}
\end{equation}
\end{footnotesize}
where the covariance matrices in the last row are related to the angular power spectra through
\begin{equation}
C_{f f^\prime,\theta \theta^\prime}^{j} = \sum_\ell (2\ell+1)C_\ell^j(f,f^\prime)\mathcal{P}_\ell^{\theta \theta^\prime}\, ,
\end{equation} 
with $\mathcal{P}_\ell$ the Legendre polynomials. Note that here we have assumed that the SN and the intrinsic anisotropies are uncorrelated. So, the total covariance matrix is the sum of the two covariance matrices found before, because they are uncorrelated,
\begin{equation}
\begin{split}
{\rm cov}_{\theta\theta^\prime} = \sum_{f,f^\prime}\Biggl[&\frac{1}{2\Delta f^2}{\rm Tr}\left(E^{f f^\prime}_{\theta}S_f E_{\theta^\prime}^{f^\prime f}S_{f^\prime}\right)+\\
&+\frac{1}{(2\Delta f)^2}\sum_{\theta^{\prime\prime},\theta^{\prime\prime\prime}}{\rm Tr}\left(E^{f f}_{\theta}B^{\rm KD}_{f,\theta^{\prime\prime}}\right){\rm Tr}\left(E^{f^\prime f^\prime}_{\theta^\prime}B^{\rm KD}_{f^\prime,\theta^{\prime\prime\prime}}\right)\left(\frac{C_{f f^\prime,\theta^{\prime\prime}\theta^{\prime\prime\prime}}^{\rm int}+C_{f f^\prime,\theta^{\prime\prime}\theta^{\prime\prime\prime}}^{\rm SN}}{\mathcal{E}_f^{\rm KD}\mathcal{E}^{\rm KD}_{f^\prime}} \right)\Biggl]\, .
\end{split}
\end{equation}
\begin{comment}
We know that the angular power spectrum of SN is constant, because the covariance matrix is proportional to $\delta_{\theta \theta^\prime}$, therefore we write the previous expression as
\begin{equation}
\begin{split}
{\rm cov}_{\rm tot,\theta\theta^\prime} = \sum_{f,f^\prime}\Biggl[&\frac{1}{2\Delta f^2}{\rm Tr}\left(E^{f f^\prime}_{\theta}S_f E_{\theta^\prime}^{f^\prime f}S_{f^\prime}\right)+\delta_{\theta \theta^\prime}C_{\rm piv,\theta\theta}^{\rm KD}+\\
&+\frac{1}{(2\Delta f)^2}\sum_{f,f^\prime,\theta^{\prime\prime}}{\rm Tr}\left(E^{f f}_{\theta}B^{\rm KD}_{f,\theta^{\prime\prime}}\right){\rm Tr}\left(E^{f^\prime f^\prime}_{\theta^\prime}B^{\rm KD}_{f^\prime,\theta^{\prime\prime}}\right)\left(\frac{C_{f f^\prime,\theta^{\prime\prime}\theta^{\prime\prime\prime}}^{\rm int}+C_{f f^\prime}^{\rm SN}}{\mathcal{E}_f^{\rm KD}\mathcal{E}^{\rm KD}_{f^\prime}} \right)\Biggl]\, .
\end{split}
\end{equation}
\end{comment}
From now on we neglect the intrinsic anisotropies for three reasons:
\begin{itemize}
\item the intrinisc anisotropies are at least two orders of magnitude smaller than the SN;
\item the intrisic anisotropies have almost the same frequency dependence of the SN. Therefore if rhe SN will be reduced by this component separation, probably also the intrisic anisotropies will be;
\item from a numerical point of view, we can compute the covariance matrix of the SN for many frequencies in a fast way. However, to compute the covariance matrix of the intrinsic anisotropies, would require heavy computational power. This would not have a large impact on the technique that we are proposing and would be beyond the scope of this paper.
\end{itemize}
By neglecting the instrinsic anisotropies the computation is simplified, because the SN is proportional to $\delta_{\theta^{\prime\prime}\theta^{\prime\prime\prime}}$ (the angular power spectrum is constant in $\ell$), therefore the covariance matrix becomes
\begin{equation}
\begin{split}
{\rm cov}_{\theta\theta^\prime} = \frac{1}{2\Delta f^2}\sum_{f,f^\prime}\Biggl[&{\rm Tr}\left(E^{f f^\prime}_{\theta}S_f E_{\theta^\prime}^{f^\prime f}S_{f^\prime}\right)+\frac{1}{2}\sum_{\theta^{\prime\prime}}{\rm Tr}\left(E^{f f}_{\theta}B^{\rm KD}_{f,\theta^{\prime\prime}}\right){\rm Tr}\left(E^{f^\prime f^\prime}_{\theta^\prime}B^{\rm KD}_{f^\prime,\theta^{\prime\prime}}\right)\frac{C_{f f^\prime}^{\rm SN}}{\mathcal{E}_f^{\rm KD}\mathcal{E}^{\rm KD}_{f^\prime}}\Biggl]\, .
\end{split}
\end{equation}
Using a Lagrange multiplier we minimize the covariance,
\begin{equation}
\mathcal{L} = {\rm cov}_{\theta\theta^\prime}-\lambda_\theta\left[\frac{1}{2\Delta f}\sum_f {\rm Tr}\left(E^{ff}_{\theta}B^{\rm KD}_{f\theta^\prime}\right)-\delta_{\theta \theta^\prime}\right]\, .
\end{equation}
By imposing that the derivative of $\mathcal{L}$ w.r.t. $E^{f f^\prime}_{\theta^\prime,AB}$ is zero we have 
\begin{equation}
\begin{split}
\sum_{C,D}S_f^{AC}E^{f^\prime f}_{\theta,CD}S_{f^\prime}^{DB}+&\frac{\delta_{f f^\prime}}{2}\sum_{f^{\prime\prime},\theta^{\prime\prime}}B^{\rm KD,AB}_{f,\theta^{\prime\prime}}{\rm Tr}\left(E^{f^{\prime\prime} f^{\prime\prime}}_{\theta}B^{\rm KD}_{f^{\prime\prime},\theta^{\prime\prime}}\right)\frac{C_{f f^{\prime\prime}}^{\rm SN}}{\mathcal{E}_f^{\rm KD}\mathcal{E}^{\rm KD}_{f^{\prime\prime}}}-\Delta f\lambda_\theta \delta_{f f^\prime} B^{AB,\rm KD}_{f,\theta} = 0 \, .
\end{split}
\end{equation}
We write the equation without writing explicitly the detector indices,
\begin{equation}
S_f E_{\theta}^{f f^\prime} S_{f^\prime} + \frac{\delta_{f f^\prime}}{2}\sum_{f^{\prime\prime},\theta^{\prime\prime}}B_{f,\theta^{\prime\prime}}^{\rm KD} {\rm Tr}\left(E^{f^{\prime\prime}f^{\prime\prime}}_\theta B^{\rm KD}_{f^{\prime\prime},\theta^{\prime\prime}}\right)\frac{C_{f f^{\prime\prime}}^{\rm SN}}{\mathcal{E}_f^{\rm KD}\mathcal{E}^{\rm KD}_{f^{\prime\prime}}}=\Delta f\lambda_\theta\delta_{f f^\prime} B^{\rm KD}_{f,\theta} \, ,
\end{equation}
When $f\neq f^\prime$ we find
\begin{equation}
S_f E_{\theta}^{f f^\prime} = 0\, ,
\end{equation}
which mean that $E_\theta^{f f^\prime}=0$ or that $E_\theta^{f f^\prime}$ belongs to the Kernel of $S_f$. \\
For the moment, we are interested in $f=f^\prime$, therefore we find
\begin{equation}
E_{\theta}^{f f}+ \frac{1}{2}\sum_{f^{\prime\prime},\theta^{\prime\prime}}S_f^{-1}B_{f,\theta^{\prime\prime}}^{\rm KD}S_f^{-1} {\rm Tr}\left(E^{f^{\prime\prime}f^{\prime\prime}}_\theta B^{\rm KD}_{f^{\prime\prime},\theta^{\prime\prime}}\right)\frac{C_{f f^{\prime\prime}}^{\rm SN}}{\mathcal{E}_f^{\rm KD}\mathcal{E}^{\rm KD}_{f^{\prime\prime}}}=\Delta f\lambda_\theta S_f^{-1} B^{\rm KD}_{f,\theta}S_f^{-1} \, .
\end{equation}
Motivated by Figure \ref{all_noises_figure}, we solve this equation in perturbation theory, expanding at first order in $C^{\rm SN}_{f f^{\prime\prime}}$.
The zero order solution is 
\begin{equation}
E^{ff\, (0)}_\theta = \Delta f \lambda_\theta S_f^{-1}B_{f,\theta}^{\rm KD}S_f^{-1}\, .
\end{equation}
We substitute this solution in the trace, finding that the first order solution is
\begin{equation}
E^{ff\, (1)}_\theta =-\frac{1}{2} \Delta f \lambda_\theta \sum_{f^{\prime\prime},\theta^{\prime\prime}}S_f^{-1}B_{f,\theta^{\prime\prime}}^{\rm KD}S_f^{-1}{\rm Tr}\left(S_{f^{\prime\prime}}^{-1}B_{f^{\prime\prime}\theta}^{\rm KD}S_{f^{\prime\prime}}^{-1}B_{f^{\prime\prime},\theta^{\prime\prime}}^{\rm KD}\right)\frac{C_{f f^{\prime\prime}}^{\rm SN}}{\mathcal{E}_f^{\rm KD}\mathcal{E}_{f^{\prime\prime}}^{\rm KD}}\, .
\end{equation}
The full solution is simply given by the sum of the two contributions,
\begin{equation}
E^{ff}_\theta = \lambda_\theta\,\Delta f \left[ S_f^{-1}B_{f,\theta}^{\rm KD}S_f^{-1}-\frac{1}{2}\sum_{f^{\prime\prime},\theta^{\prime\prime}}S_f^{-1}B_{f,\theta^{\prime\prime}}^{\rm KD}S_f^{-1}{\rm Tr}\left(S_{f^{\prime\prime}}^{-1}B_{f^{\prime\prime}\theta}^{\rm KD}S_{f^{\prime\prime}}^{-1}B_{f^{\prime\prime},\theta^{\prime\prime}}^{\rm KD}\right)\frac{C_{f f^{\prime\prime}}^{\rm SN}}{\mathcal{E}_f^{\rm KD}\mathcal{E}_{f^{\prime\prime}}^{\rm KD}}\right]\, .
\end{equation}
To find the parameter $\lambda_\theta$ we use the condition given by the Lagrange multiplier with $\theta = \theta^\prime$,
\begin{equation}
\lambda_\theta = & \frac{2}{\sum_f{\rm Tr}\left(S_f^{-1}B_{f,\theta}^{\rm KD}S_f^{-1}B_{f,\theta}^{\rm KD}\right)}+\sum_{f^{\prime\prime},\theta^{\prime\prime}}\frac{\sum_f{\rm Tr}\left(S_f^{-1}B_{f,\theta^{\prime\prime}}^{\rm KD}S_f^{-1}B_{f,\theta}^{\rm KD}\right){\rm Tr}\left(S_{f^{\prime\prime}}^{-1}B_{f^{\prime\prime}\theta}^{\rm KD}S_{f^{\prime\prime}}^{-1}B_{f^{\prime\prime},\theta^{\prime\prime}}^{\rm KD}\right)}{\left[\sum_f{\rm Tr}\left(S_f^{-1}B_{f,\theta}^{\rm KD}S_f^{-1}B_{f,\theta}^{\rm KD}\right)\right]^2}\frac{C_{f f^{\prime\prime}}^{\rm SN}}{\mathcal{E}_f^{\rm KD}\mathcal{E}_{f^{\prime\prime}}^{\rm KD}}\, ,
\end{equation}
and the final expression for the weights to give to the signals measured at interferometers are
\begin{small}
\begin{equation}
\begin{split}
\frac{E^{ff}_\theta}{\Delta f} = &  \left[\frac{2}{\sum_f{\rm Tr}\left(S_f^{-1}B_{f,\theta}^{\rm KD}S_f^{-1}B_{f,\theta}^{\rm KD}\right)}+\sum_{f^{\prime\prime},\theta^{\prime\prime}}\frac{\sum_f{\rm Tr}\left(S_f^{-1}B_{f,\theta^{\prime\prime}}^{\rm KD}S_f^{-1}B_{f,\theta}^{\rm KD}\right){\rm Tr}\left(S_{f^{\prime\prime}}^{-1}B_{f^{\prime\prime}\theta}^{\rm KD}S_{f^{\prime\prime}}^{-1}B_{f^{\prime\prime},\theta^{\prime\prime}}^{\rm KD}\right)}{\left[\sum_f{\rm Tr}\left(S_f^{-1}B_{f,\theta}^{\rm KD}S_f^{-1}B_{f,\theta}^{\rm KD}\right)\right]^2}\frac{C_{f f^{\prime\prime}}^{\rm SN}}{\mathcal{E}_f^{\rm KD}\mathcal{E}_{f^{\prime\prime}}^{\rm KD}}\right]\\
&\left[S_f^{-1}B_{f,\theta}^{\rm KD}S_f^{-1}-\frac{1}{2}\sum_{f^{\prime\prime},\theta^{\prime\prime}}S_f^{-1}B_{f,\theta^{\prime\prime}}^{\rm KD}S_f^{-1}{\rm Tr}\left(S_{f^{\prime\prime}}^{-1}B_{f^{\prime\prime}\theta}^{\rm KD}S_{f^{\prime\prime}}^{-1}B_{f^{\prime\prime},\theta^{\prime\prime}}^{\rm KD}\right)\frac{C_{f f^{\prime\prime}}^{\rm SN}}{\mathcal{E}_f^{\rm KD}\mathcal{E}_{f^{\prime\prime}}^{\rm KD}}\right]= \\
= & \frac{2S_f^{-1}B_{f,\theta}^{\rm KD}S_f^{-1}}{\sum_{f^\prime}{\rm Tr}\left(S_{f^\prime}^{-1}B_{f^\prime,\theta}^{\rm KD}S_{f^\prime}^{-1}B_{f^\prime,\theta}^{\rm KD}\right)}+\\
&+S_f^{-1}B_{f,\theta}^{\rm KD}S_f^{-1}\sum_{f^\prime,f^{\prime\prime},\theta^{\prime\prime}}\frac{{\rm Tr}\left(S_{f^\prime}^{-1}B_{f^\prime,\theta^{\prime\prime}}^{\rm KD}S_{f^\prime}^{-1}B_{f^\prime,\theta}^{\rm KD}\right){\rm Tr}\left(S_{f^{\prime\prime}}^{-1}B_{f^{\prime\prime}\theta}^{\rm KD}S_{f^{\prime\prime}}^{-1}B_{f^{\prime\prime},\theta^{\prime\prime}}^{\rm KD}\right)}{\left[\sum_{f^\prime}{\rm Tr}\left(S_{f^\prime}^{-1}B_{f^\prime,\theta}^{\rm KD}S_{f^\prime}^{-1}B_{f^\prime,\theta}^{\rm KD}\right)\right]^2}\frac{C_{f^\prime f^{\prime\prime}}^{\rm SN}}{\mathcal{E}_{f^\prime}^{\rm KD}\mathcal{E}_{f^{\prime\prime}}^{\rm KD}}+\\
&+(-1)\sum_{f^{\prime\prime},\theta^{\prime\prime}}S_f^{-1}B_{f,\theta^{\prime\prime}}^{\rm KD}S_f^{-1}\frac{{\rm Tr}\left(S_{f^{\prime\prime}}^{-1}B_{f^{\prime\prime}\theta}^{\rm KD}S_{f^{\prime\prime}}^{-1}B_{f^{\prime\prime},\theta^{\prime\prime}}^{\rm KD}\right)}{\sum_{f^\prime}{\rm Tr}\left(S_{f^\prime}^{-1}B_{f^\prime,\theta}^{\rm KD}S_{f^\prime}^{-1}B_{f^\prime,\theta}^{\rm KD}\right)}\frac{C_{f f^{\prime\prime}}^{\rm SN}}{\mathcal{E}_f^{\rm KD}\mathcal{E}_{f^{\prime\prime}}^{\rm KD}}\, .
\end{split}
\end{equation}
\end{small}
The covariance matrix up to first order in $C^{\rm SN}_{f f^{\prime\prime}}$ is therefore
\begin{small}
\begin{equation}
\begin{split}
{\rm cov}_{\theta\theta^\prime} =& \frac{1}{2\Delta f^2}\sum_{f,f^\prime}\Biggl[{\rm Tr}\left(E^{f f^\prime}_{\theta}S_f E_{\theta^\prime}^{f^\prime f}S_{f^\prime}\right)+\frac{1}{2}\sum_{\theta^{\prime\prime}}{\rm Tr}\left(E^{f f}_{\theta}B^{\rm KD}_{f,\theta^{\prime\prime}}\right){\rm Tr}\left(E^{f^\prime f^\prime}_{\theta^\prime}B^{\rm KD}_{f^\prime,\theta^{\prime\prime}}\right)\frac{C_{f f^\prime}^{\rm SN}}{\mathcal{E}_f^{\rm KD}\mathcal{E}^{\rm KD}_{f^\prime}}\Biggl]= \\
=& \frac{1}{\Delta f}\sum_f\Biggl\{\frac{{\rm Tr}\left(E^{ff}_\theta B^{\rm KD}_{f,\theta^\prime}\right)}{\sum_{f^\prime}{\rm Tr}\left(S_{f^\prime}^{-1}B_{f^\prime,\theta^\prime}^{\rm KD}S_{f^\prime}^{-1}B_{f^\prime,\theta^\prime}^{\rm KD}\right)}\times\\
&\hspace{2em}\times\left[1+\frac{1}{2}\sum_{f^\prime,f^{\prime\prime},\theta^{\prime\prime}}\frac{{\rm Tr}\left(S_{f^\prime}^{-1}B_{f^\prime,\theta^{\prime\prime}}^{\rm KD}S_{f^\prime}^{-1}B_{f^\prime,\theta^\prime}^{\rm KD}\right){\rm Tr}\left(S_{f^{\prime\prime}}^{-1}B_{f^{\prime\prime}\theta^\prime}^{\rm KD}S_{f^{\prime\prime}}^{-1}B_{f^{\prime\prime},\theta^{\prime\prime}}^{\rm KD}\right)}{\sum_{f^\prime}{\rm Tr}\left(S_{f^\prime}^{-1}B_{f^\prime,\theta^\prime}^{\rm KD}S_{f^\prime}^{-1}B_{f^\prime,\theta^\prime}^{\rm KD}\right)}\frac{C_{f^\prime f^{\prime\prime}}^{\rm SN}}{\mathcal{E}_{f^\prime}^{\rm KD}\mathcal{E}_{f^{\prime\prime}}^{\rm KD}}\right]+\\
&\hspace{2em}+\left(-\frac{1}{2}\right)\sum_{f^{\prime\prime},\theta^{\prime\prime}}{\rm Tr}\left(E^{ff}_\theta B_{f,\theta^{\prime\prime}}^{\rm KD}\right)\frac{{\rm Tr}\left(S_{f^{\prime\prime}}^{-1}B_{f^{\prime\prime}\theta^\prime}^{\rm KD}S_{f^{\prime\prime}}^{-1}B_{f^{\prime\prime},\theta^{\prime\prime}}^{\rm KD}\right)}{\sum_{f^\prime}{\rm Tr}\left(S_{f^\prime}^{-1}B_{f^\prime,\theta^\prime}^{\rm KD}S_{f^\prime}^{-1}B_{f^\prime,\theta^\prime}^{\rm KD}\right)}\frac{C_{f f^{\prime\prime}}^{\rm SN}}{\mathcal{E}_f^{\rm KD}\mathcal{E}_{f^{\prime\prime}}^{\rm KD}}+\\
&\hspace{2em}+\frac{1}{4}\sum_{f^\prime\theta^{\prime\prime}}\frac{2{\rm Tr}\left(S_f^{-1}B^{\rm KD}_{f,\theta}S_f^{-1}B^{\rm KD}_{f,\theta^{\prime\prime}}\right)}{\sum_{f^\prime}{\rm Tr}\left(S_{f^\prime}^{-1}B_{f^\prime,\theta}^{\rm KD}S_{f^\prime}^{-1}B_{f^\prime,\theta}^{\rm KD}\right)}\frac{2{\rm Tr}\left(S_{f^\prime}^{-1}B^{\rm KD}_{f^\prime\theta^\prime}S_{f^\prime}^{-1}B^{\rm KD}_{f^\prime,\theta^{\prime\prime}}\right)}{\sum_{f^\prime}{\rm Tr}\left(S_{f^\prime}^{-1}B_{f^\prime,\theta^\prime}^{\rm KD}S_{f^\prime}^{-1}B_{f^\prime,\theta^\prime}^{\rm KD}\right)}\frac{C_{f f^\prime}^{\rm SN}}{\mathcal{E}_f^{\rm KD}\mathcal{E}^{\rm KD}_{f^\prime}}+
\Biggl\}= \\
=& \frac{2\delta_{\theta\theta^\prime}}{\sum_{f^\prime}{\rm Tr}\left(S_{f^\prime}^{-1}B_{f^\prime,\theta}^{\rm KD}S_{f^\prime}^{-1}B_{f^\prime,\theta}^{\rm KD}\right)}+\\
&+\delta_{\theta\theta^\prime}\sum_{f^\prime,f^{\prime\prime},\theta^{\prime\prime}}\frac{{\rm Tr}\left(S_{f^\prime}^{-1}B_{f^\prime,\theta^{\prime\prime}}^{\rm KD}S_{f^\prime}^{-1}B_{f^\prime,\theta^\prime}^{\rm KD}\right){\rm Tr}\left(S_{f^{\prime\prime}}^{-1}B_{f^{\prime\prime}\theta^\prime}^{\rm KD}S_{f^{\prime\prime}}^{-1}B_{f^{\prime\prime},\theta^{\prime\prime}}^{\rm KD}\right)}{\left[\sum_{f^\prime}{\rm Tr}\left(S_{f^\prime}^{-1}B_{f^\prime,\theta^\prime}^{\rm KD}S_{f^\prime}^{-1}B_{f^\prime,\theta^\prime}^{\rm KD}\right)\right]^2}\frac{C_{f^\prime f^{\prime\prime}}^{\rm SN}}{\mathcal{E}_{f^\prime}^{\rm KD}\mathcal{E}_{f^{\prime\prime}}^{\rm KD}}\, .
\end{split}
\end{equation}
\end{small}
The minimum covariance we will have in estimating the kinetic dipole is
\begin{small}
\begin{equation}
{\rm cov}_{\theta\theta^\prime}=\frac{2\delta_{\theta\theta^\prime}}{\sum_{f}{\rm Tr}\left(S_{f}^{-1}B_{f,\theta}^{\rm KD}S_{f}^{-1}B_{f,\theta}^{\rm KD}\right)}+\delta_{\theta\theta^\prime}\sum_{f,f^\prime,\theta^{\prime\prime}}\frac{{\rm Tr}\left(S_{f}^{-1}B_{f,\theta^{\prime\prime}}^{\rm KD}S_{f}^{-1}B_{f,\theta^\prime}^{\rm KD}\right){\rm Tr}\left(S_{f^{\prime}}^{-1}B_{f^{\prime}\theta^\prime}^{\rm KD}S_{f^{\prime}}^{-1}B_{f^{\prime},\theta^{\prime\prime}}^{\rm KD}\right)}{\left[\sum_{f}{\rm Tr}\left(S_{f}^{-1}B_{f,\theta}^{\rm KD}S_{f}^{-1}B_{f,\theta}^{\rm KD}\right)\right]^2}\frac{C_{f f^{\prime}}^{\rm SN}}{\mathcal{E}_{f}^{\rm KD}\mathcal{E}_{f^{\prime}}^{\rm KD}}\, .
\end{equation}
\end{small}
The first term is the standard term due to instrumental noise, while the second one is the term due to SN, that is maximimally reduced by the weights in $f$, $f^\prime$ we have chosen. \\
To connect the covariance of $\hat{I}_{\rm piv}$ to the covariance of $\delta_{\rm AGWB}^{\rm KD}(f_{\rm piv})$ we use Eq. \eqref{I_Omega_Equation},
\begin{equation}
{\rm cov}_{\theta\theta^{\prime}}^{\rm \delta_{\rm AGWB}}=\left( \frac{1}{\bar{\Omega}_{\rm AGWB}(f_{\rm piv})}\frac{4\pi f^3}{3H_0^2}\right)^2{\rm cov}_{\theta\theta^\prime}\, .
\end{equation}
Keep in mind that, according to the definitions we have used here, the covariance matrix associated to SN is the covariance matrix of the intensity, which is related to the covariance matrix of the density contrast through
\begin{equation}
C_{f f^\prime}^{\rm SN} = \left(\bar{\Omega}_{\rm AGWB}(f_{\rm piv})\frac{3H_0^2}{4\pi f^3}\right)^2C_{f f^\prime}^{\rm SN,\delta_{\rm AGWB}}\, .
\end{equation}
We do not follow here the approach of~\cite{Alonso:2020rar}, where an angular power spectrum of the noise is computed, because we want to take into account for inhomogeneities in noise $m$-modes, measuring the direction of the kinematic dipole. \\
First of all, what we have done until now has been done for a single timeframe. We would like to compute the total noise after $T_{\rm obs = 10}\, \rm yr$ of observations. In~\cite{LISACosmologyWorkingGroup:2022kbp} it is discussed very well the effects of rotation on the detector response. For the moment we neglect the effect of rigid rotations and we divide the covariance we have found by $T_{\rm obs}$,
\begin{equation}
{\rm cov}^{\rm \delta_{\rm AGWB},tot}_{\theta\theta^\prime} =\frac{1}{T_{\rm obs}}{\rm cov}_{\theta\theta^{\prime}}^{\rm \delta_{\rm AGWB}}\, .
\end{equation}
The computation of the error on our dipole estimate is performed by using
\begin{equation}
{\rm cov}_{1m,1m^\prime} = \sum_\theta Y_{1m}^\theta Y_{1m^\prime}^{\theta,*}{\rm cov}^{\rm \delta_{\rm AGWB},tot}_{\theta\theta} \Delta\Omega^2\, .
\end{equation}
In the case of a monopole amplitude $\bar{\Omega}_{\rm AGWB}(f=50\, \rm Hz)$ we find
\begin{equation}
{\rm cov}_{1m,1m^\prime} =
\begin{pmatrix}
8.2\times 10^{-7} & 1.1\times 10^{-8} & 2.0\times 10^{-7} \\
1.1\times10^{-8} & 3.1\times 10^{-6} & -1.1\times 10^{-8}\\
2.0 \times 10^{-7} & -1.1\times 10^{-8} & 8.2\times 10^{-7}
\end{pmatrix}\, .
\end{equation}
Just to give an order of magnitude of the error on the dipole we use
\begin{equation}
\sigma_{d_x} = \frac{1}{2}\sqrt{\frac{3}{\pi}}{\rm cov}_{10,10^\prime}\approx 0.0004\, .
\end{equation}
