# Supplementary material for: The Dipole of the Astrophysical Gravitational-Wave Background
Source: arXiv:2206.02747 source file (2022-12-05)
Supplement: Supplementary file 8 [file SN.tex]

\label{Shot Noise}

%\subsubsection{Shot Noise}
%\label{Shot Noise Computation}

Since the AGWB is generated by the superposition of unresolved astrophysical sources, it is naturally affected by SN, because the sources are discrete events which follow a Poisson distribution~\cite{}. The variance associated to the expected number of processes corresponds exactly to the SN. Let's consider a generic Poisson process, where in a volume $\delta V$  the expected number of objects is $\bar{n}\delta V$. The probability of counting $N_i$ objects in $\delta V$ is a Poisson distribution\footnote{For the last relation we have used
\begin{equation}
\langle (N_i-\bar{n}\delta V)(N_j-\bar{n}\delta V)\rangle = \delta(\hat{n}_i-\hat{n}_j) \bar{n}\delta V\, .
\end{equation}
},
\begin{equation}
\begin{split}
p(N_i) =&  \frac{\left(\bar{n}\delta V\right)^{N_i}}{N_i!}e^{-\bar{n}\delta V}\, , \\
\langle N_i \rangle =& \bar{n}\delta V\, , \\
\langle N_i N_j \rangle = & \left(\bar{n}\delta V\right)^2+\bar{n}\delta V\delta(\hat{n}_i-\hat{n}_j)\, ,
\end{split}
\label{Poisson_Distribution_Equation}
\end{equation}
where $i$, $j$ label the bins of the survey, i.e. the directions of observation. Note that the correlation term $\langle N_i N_j\rangle$ has a term proportional to $\delta_{ij}$ which is exactly the variance of a Poisson distribution, and another term which represents $\langle N_i\rangle \langle N_j\rangle = (\bar{n}\delta V) ^2$.\\
In the case of the merging of BBHs we have two independent Poisson distributions to consider, the first one refers to the number of mergers per halo of a given mass at a given redshift, while the second one to the number of halos of a given mass at a given redshift~\cite{}.\\
The distribution of $N_h(M_h,z)$ is characterized by a mean value $\bar{N}_h(M_h,z)$, and the number of merger per halo, $N_{{\rm GW}|h}(M_h,z)$, is characterized by $\bar{N}_{{\rm GW}|h}(M_h,z)$. In a volume $\delta V$ with $N_h$ halos the total number of mergers is 
\begin{equation}
N_{\rm GW} = \sum_{i=1}^{N_h} N_{{\rm GW}|h}\, .
\end{equation}
$N_{\rm GW}$ is described by a compound Poisson distribution, because it is the sum of uncorrelated, Poisson-distributed, random variables. \\
In Appendix \ref{Compound Poisson Distribution}, we show that the mean and the covariance of this kind of process are 
\begin{equation}
\begin{split}
\langle N_{\rm GW}\rangle =&  \bar{N}_h\bar{N}_{{\rm GW}|h}\, , \\
\langle N_{\rm GW}^2\rangle = & \bar{N}_h \left(\bar{N}_{{\rm GW}|h}+\bar{N}_{{\rm GW}|h}^2\right)\, .
\end{split}
\end{equation}
In our case, $\bar{N}_h$ is the average number of halos at the redshift at which the binary formed, $z_f=z_f[t(z)-t_d]$,
\begin{equation}
\bar{N}_h = \frac{dn}{dM_h}(M_h,z_f)\, .
\end{equation}
The mean number of GW events per halo is nothing but the merger rate of objects per halo, times the probability of having a merger after a time delay $t_d$ w.r.t. the formation of the binary, and times the observation time,
\begin{equation}
\bar{N}_{GW|h} = p(t_d)\mathcal{A}_{\rm LIGO}\langle {\rm SFR}(M_h,z_d)\rangle_{\rm SF}T_{\rm obs}\frac{\ud V}{\ud z\ud \Omega}\, ,
\end{equation} 
where $\mathcal{A}_{\rm LIGO}$ is the LIGO normalization on the local merger rate and $dV/dz$ is the analogous of the $\delta V$ term introduced at the beggining of this section. \\
The AGWB anisotropies are described by
\begin{equation}
\begin{split}
\delta_{\rm AGWB}(\hat{n},f_o) =\frac{1}{\bar{\Omega}_{\rm AGWB}T_{\rm obs}} \frac{f_o}{\rho_c c^2}\int& \frac{dz}{H(z)(1+z)}\frac{1}{\frac{\ud V}{\ud z\ud \Omega}}\frac{\ud E}{\ud \Omega_e \ud f_e}(z,f_o)w^{\rm DET}(z)\int dM_h\times \\
& \int dt_d p(t_d) \frac{dn}{dM_h}(M_h,z)\mathcal{A}_{\rm LIGO}\langle {\rm SFR}(M_h,z_d)\rangle_{\rm SF}T_{\rm obs}\frac{\ud V}{\ud z\ud \Omega}\, . 
\end{split}
\end{equation}
Since the fluctuations due to SN are uncorrelated with fluctuations due to cosmological perturbations, there is no cross-correlation between the SN and the intrinsic anisotropies. The only contribution given by SN is
\begin{equation}
\begin{split}
C_\ell^{\rm AGWB,SN}=&\langle \delta_{\rm AGWB}^2\rangle_{\rm SN} =\\
=&\frac{1}{\bar{\Omega}^2_{\rm AGWB}T^2_{\rm obs}} \frac{f^2_o}{\rho_c^2 c^4}\int \frac{dz}{H^2(z)(1+z)^2}\left(\frac{1}{\frac{\ud V}{\ud z\ud \Omega}}\frac{\ud E}{\ud \Omega_e\ud f_e}(z,f_o)w^{\rm DET}(z)\right)^2\int dM_h\times \\
& \int dt_d \frac{dn}{dM_h}(M_h,z)\biggl[ p(t_d)\mathcal{A}_{\rm LIGO}\langle {\rm SFR}(M_h,z_d)\rangle_{\rm SF}T_{\rm obs}\frac{\ud V}{\ud z\ud \Omega}+\\
&\hspace{10em}+\left( p(t_d)\mathcal{A}_{\rm LIGO}\langle {\rm SFR}(M_h,z_d)\rangle_{\rm SF}T_{\rm obs}\frac{\ud V}{\ud z\ud \Omega}\right)^2\biggl]\, . 
\end{split}
\label{equazione_calcolo_shot_noise}
\end{equation}
For $T_{\rm obs} = 10\, {\rm yr}$, at $f_o=50\, \rm Hz$, $N_\ell^{\rm SN}\approx 7\times 10^{-3}$. This means that it is at least one order of magnitude larger than the kinematic dipole and three orders of magnitude larger than the intrinsic dipole. For completeness, I have shown the dependence of SN on the observed frequency of the AGWB anisotropies in Figure \ref{all_dipoles_figure}. The result I have found is consistent with~\cite{Jenkins:2019uzp,Bellomo:2021mer}.\\
\begin{figure}
\centering
\includegraphics[scale=0.5]{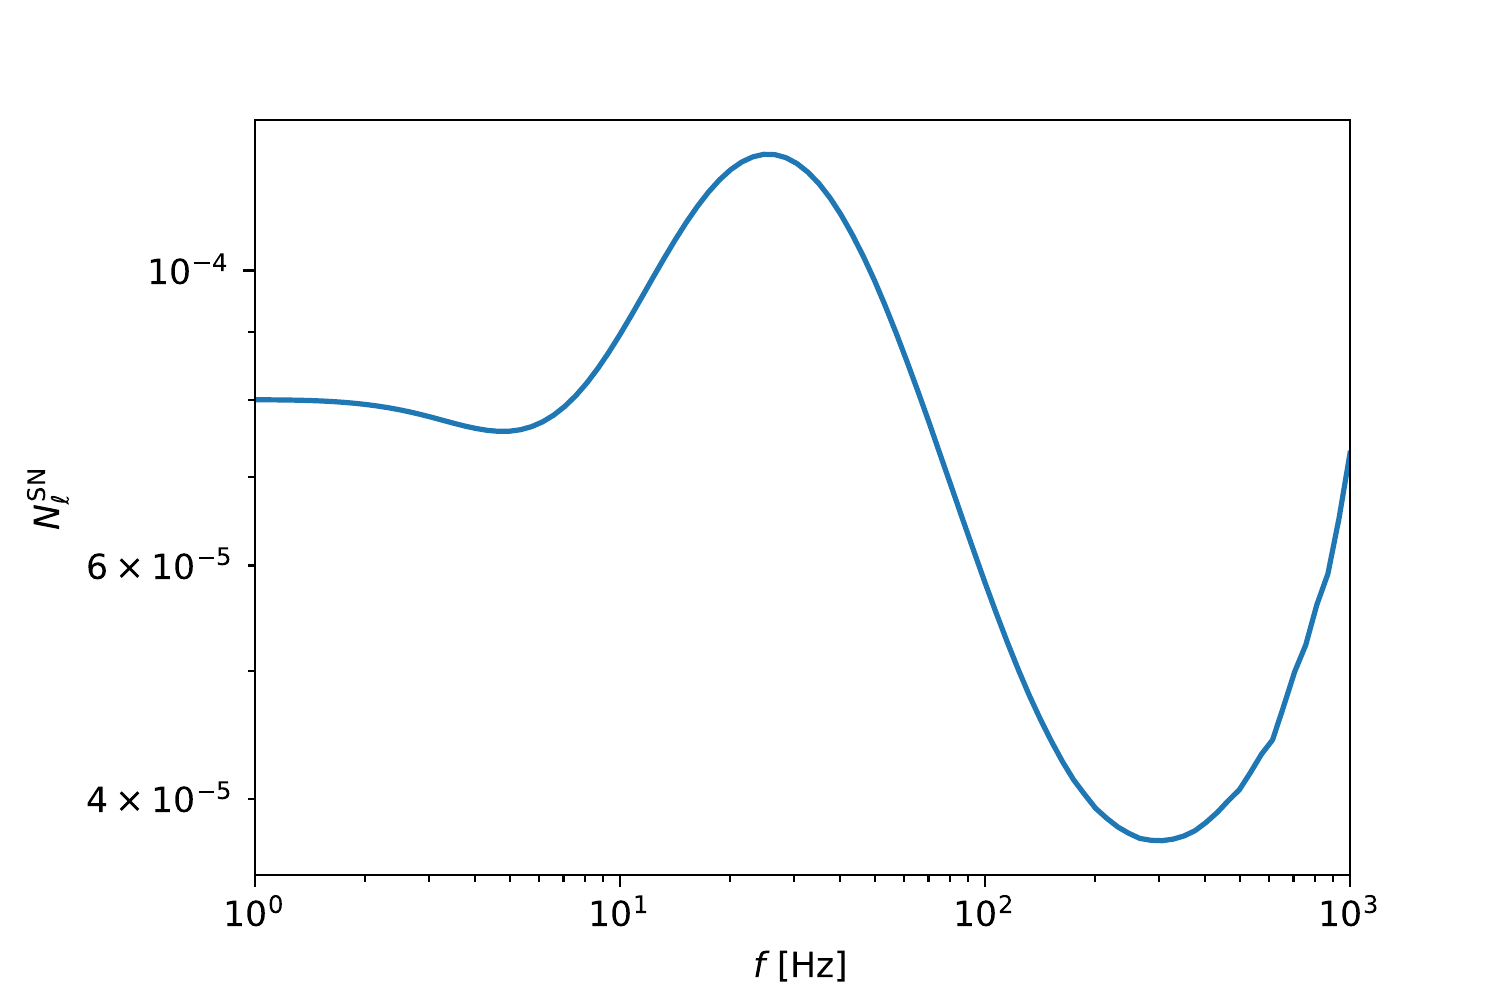}
\caption{Plot of the angular power spectrum of the SN of BBHs at different frequencies.}
\label{sn_vs_fr_figure}
\end{figure}
There are several strategies to reduce SN. The first one exploits cross-correlations. The cross-correlation allows in general to obtain higher SNRs w.r.t. the auto-correlation case, see for instance~\cite{Capurri:2021prz}. However, if SN is several orders of magnitude larger than the intrinsic anisotropies as in our case, it is not possible to cancel this contribution by using few tracers only. Alternatively, one could use new statistical estimators~\cite{Jenkins:2019nks}, to cancel the offset in the estimate of the angular power spectrum and to reduce as much as possible the SN.\\
In the next chapter, we will try to reduce SN order of magnitude by correlating the AGWB anisotropies at different frequencies, exploiting the different dependence on the frequency of the SN and of the intrinsic w.r.t. the kinematic dipole.
