# Supplementary material for: The Dipole of the Astrophysical Gravitational-Wave Background
Source: arXiv:2206.02747 source file (2022-12-05)
Supplement: Supplementary file 9 [file appendix_agwb_monopole.tex]

In Figure \ref{agwb_plot} we plot the AGWB which characterizes the AGWB, namely the AGWB monopole, the AGWB kernel/window function, and the evolution bias. At low frequencies we recognize in the monopole the inspiral contribution, $\bar{\Omega}_{\rm AGWB}\propto f^{2/3}$, while at higher frequencies the binaries start contributing while they are in the merger or in the ringdown stages and the spectral shape is no more a simple power law. The ‘‘double bump'' at high frequencies is due to the Power Law Plus Peak mass distribution we have used. The window function of the AGWB at low frequencies does not change with the frequency, because the dominant contribution to the background is given by the inspiral, thus any frequency dependence cancels out. At higher frequencies, the superposition of the AGWB signal from binaries at different stages of evolution generates a non-factorizable dependence on the frequencies w.r.t. the redshift. The same fact is true for the evolution bias. This property allows us to observe different kinematic dipoles at different frequencies, thus to perform component separation.
\begin{figure}
    \centering
    \includegraphics[scale=0.75]{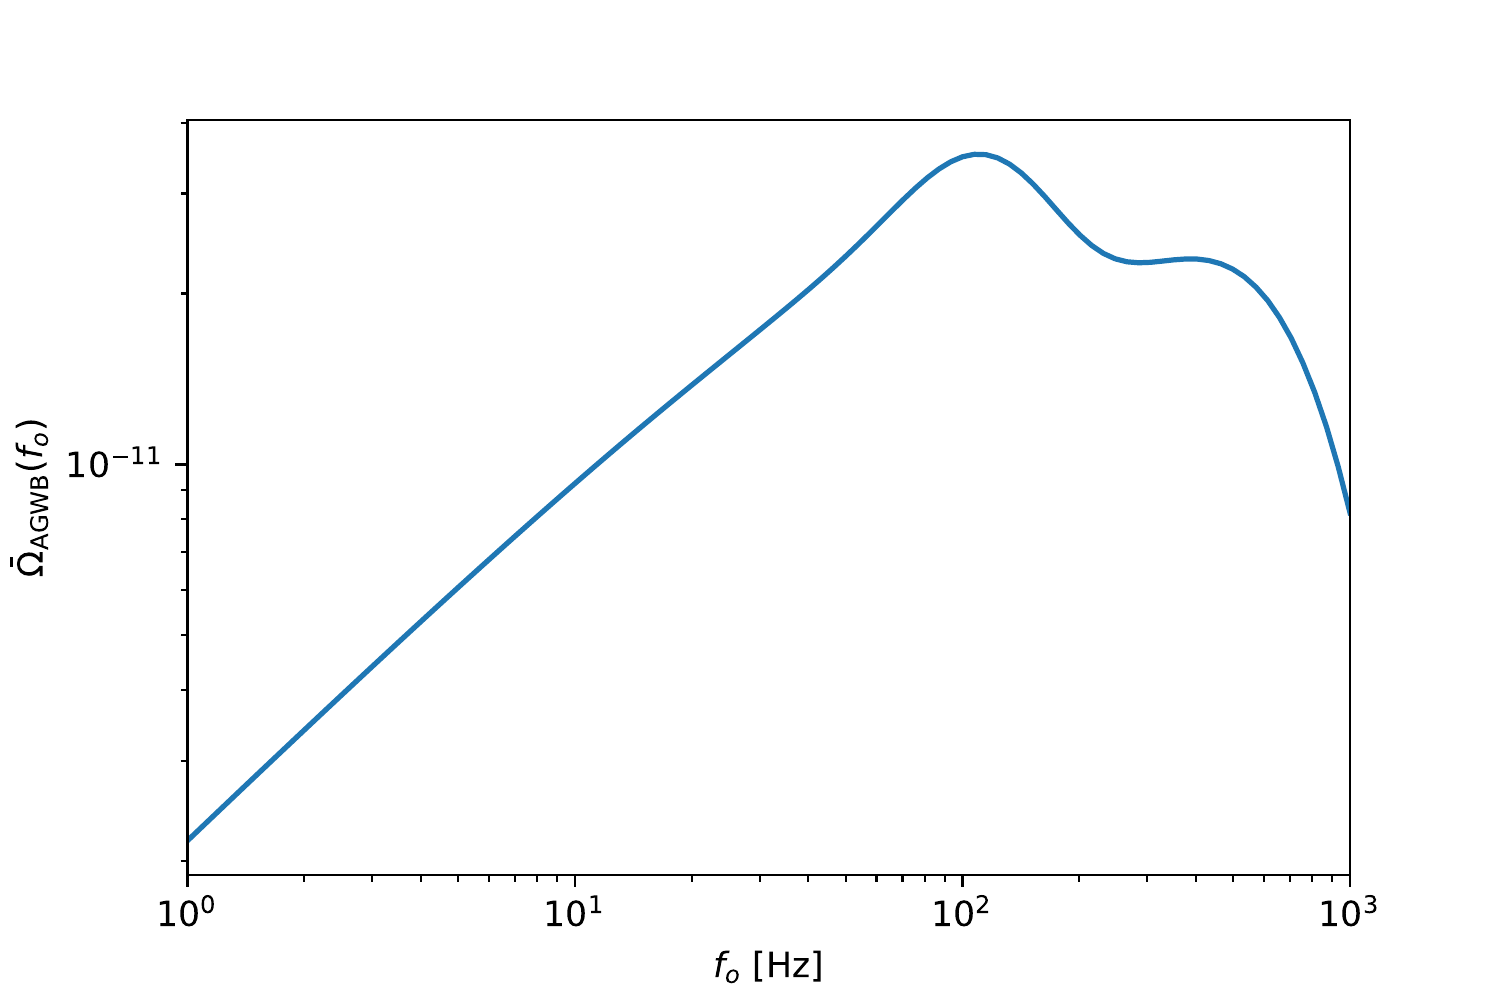}
    \includegraphics[scale=0.75]{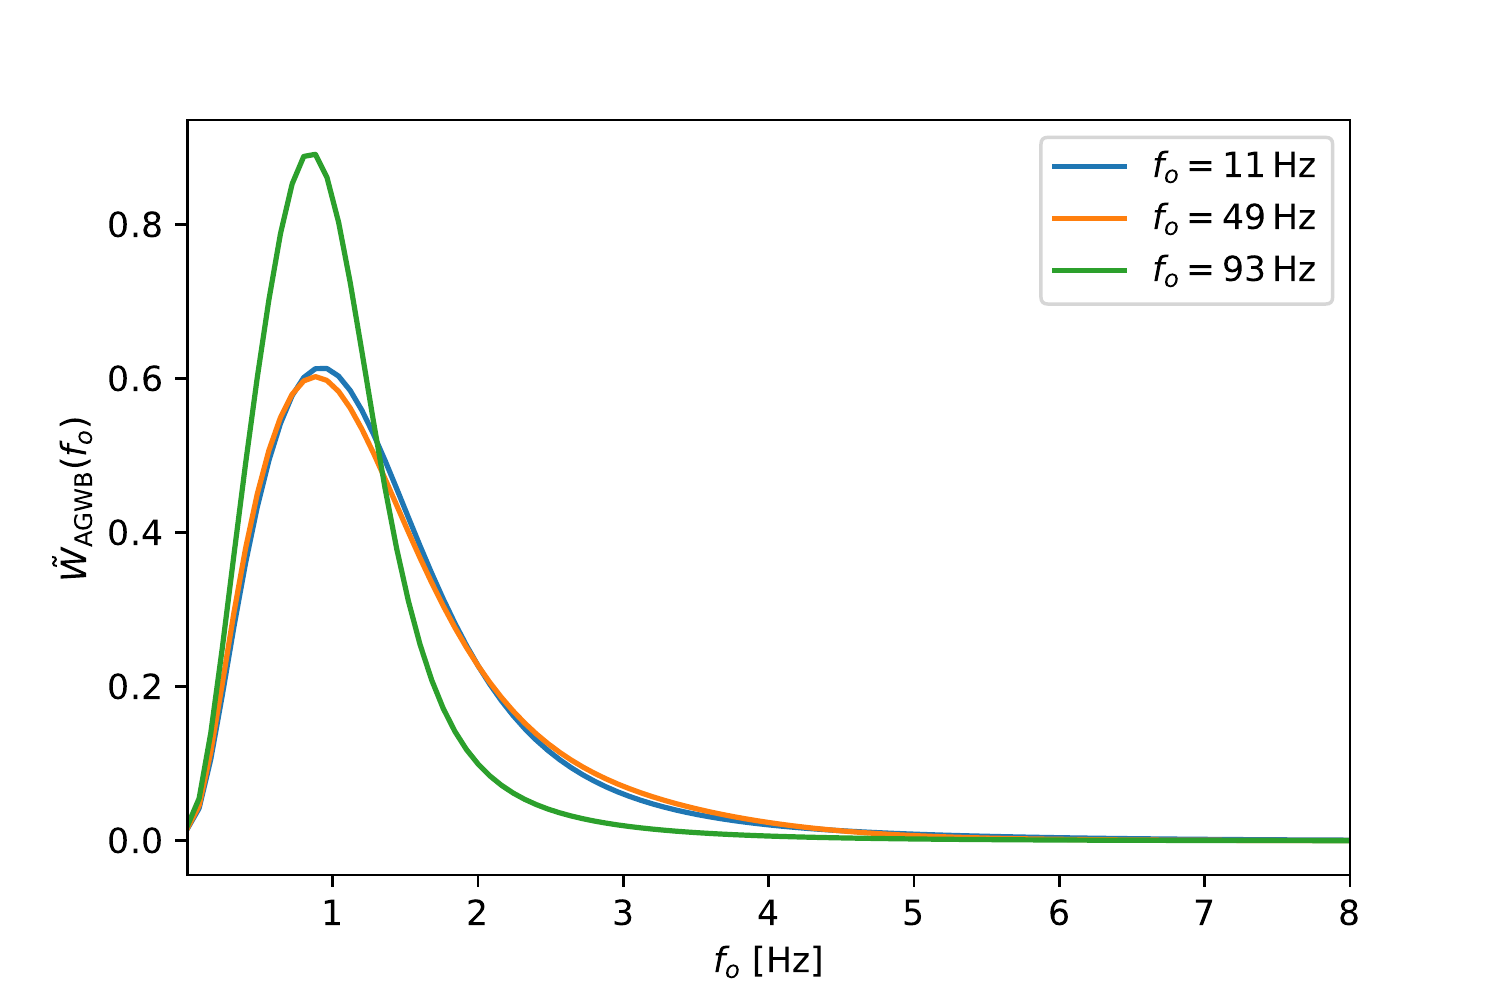}
    \includegraphics[scale=0.75]{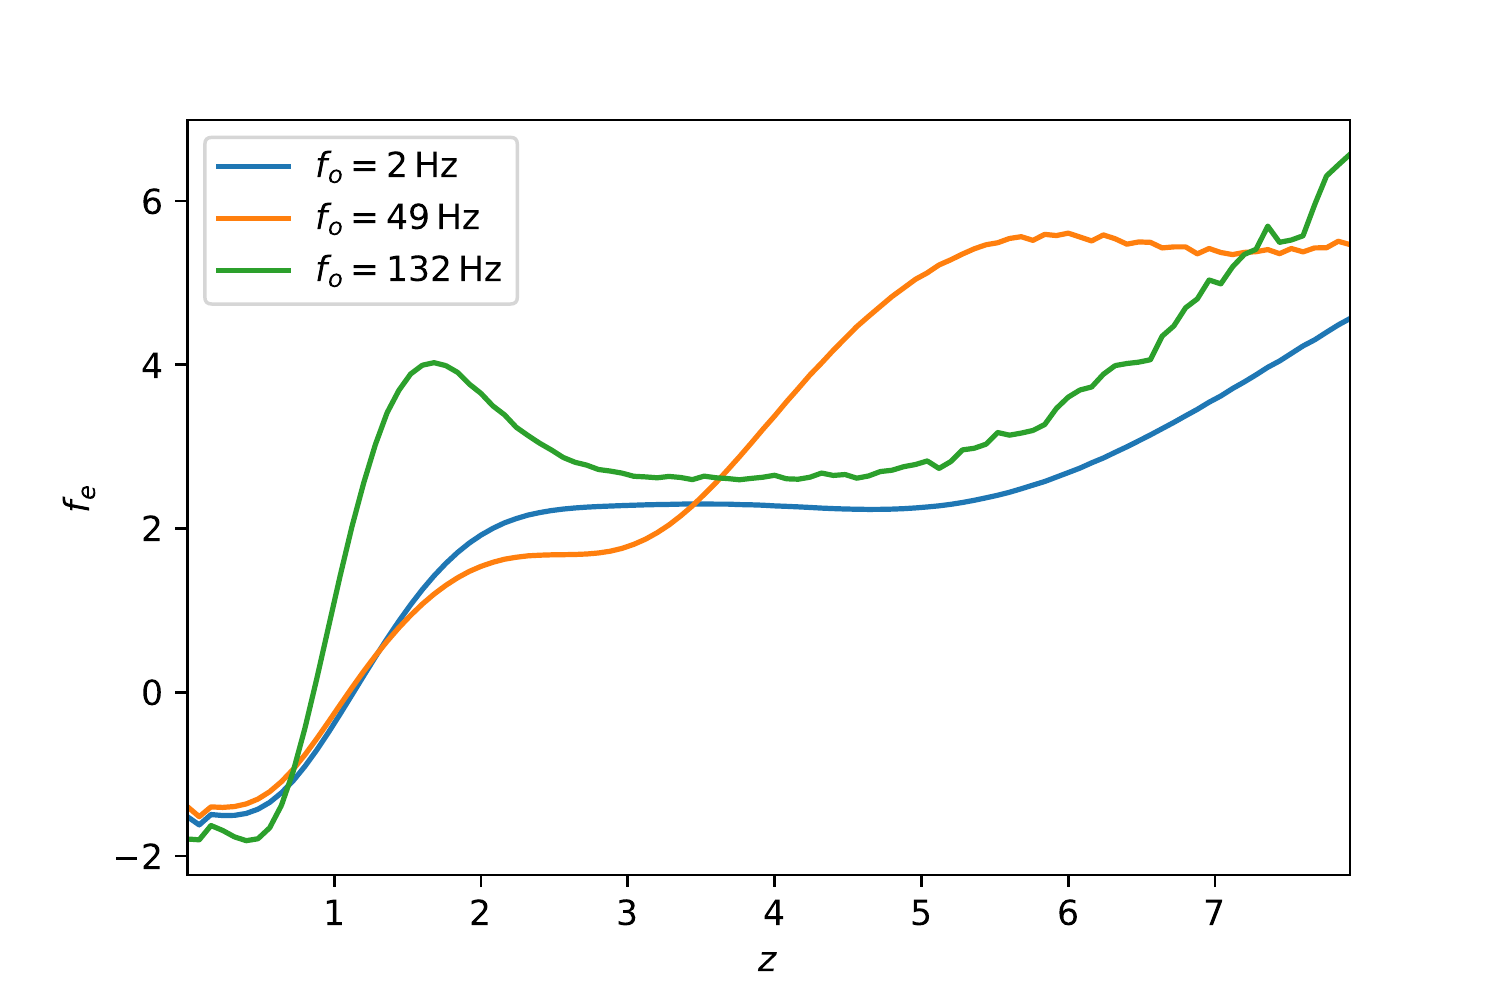}
    \caption{Upper: plot of the AGWB monopole as a function of the frequency. Middle: window function of the AGWB as a function of the redshift for different frequencies. Lower: plot of the evolution bias as a function of the redshift at different frequencies.}
    \label{agwb_plot}
\end{figure}
